# Supplementary material for: Neural reparameterization improves structural optimization
Source: arXiv:1909.04240 ancillary file (2019-09-14)
Supplement: Supplementary file 1 [file all-designs.pdf]

Table 1: Relative and absolute compliance for each of our 116 designs, for both the “typical sample” and the “best of ensemble.”

| Typical sample                                                                      |                                                                                     |                                                                                     |                                                                                     | Best of ensemble                                                                    |                                                                                      |                                                                                       |                                                                                       |
|-------------------------------------------------------------------------------------|-------------------------------------------------------------------------------------|-------------------------------------------------------------------------------------|-------------------------------------------------------------------------------------|-------------------------------------------------------------------------------------|--------------------------------------------------------------------------------------|---------------------------------------------------------------------------------------|---------------------------------------------------------------------------------------|
| CNN-LBFGS                                                                           | MMA                                                                                 | OC                                                                                  | Pixel-LBFGS                                                                         | CNN-LBFGS                                                                           | MMA                                                                                  | OC                                                                                    | Pixel-LBFGS                                                                           |
| anchored_suspended_bridge_128x128_0.1                                               |                                                                                     |                                                                                     |                                                                                     |                                                                                     |                                                                                      |                                                                                       |                                                                                       |
| 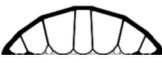   | 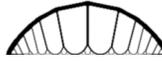   | 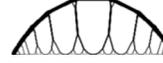   | 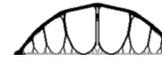   | 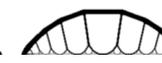   | 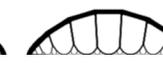   | 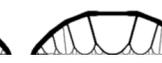   | 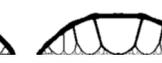   |
| 0.018 / 28.8                                                                        | 0.0 / 28.3                                                                          | 0.053 / 29.8                                                                        | 0.188 / 33.6                                                                        | 0.0 / 27.5                                                                          | 0.003 / 27.5                                                                         | 0.041 / 28.6                                                                          | 0.09 / 29.9                                                                           |
| anchored_suspended_bridge_256x256_0.05                                              |                                                                                     |                                                                                     |                                                                                     |                                                                                     |                                                                                      |                                                                                       |                                                                                       |
| 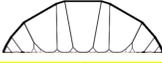   | 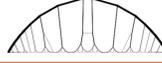   | 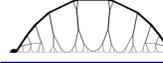   | 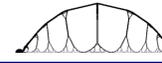   | 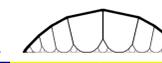   | 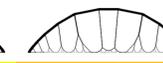   | 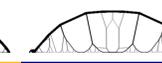   | 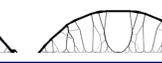   |
| 0.0 / 61.3                                                                          | 0.032 / 63.2                                                                        | 0.144 / 70.1                                                                        | 0.631 / 99.9                                                                        | 0.0 / 57.9                                                                          | 0.013 / 58.6                                                                         | 0.131 / 65.5                                                                          | 0.262 / 73.0                                                                          |
| anchored_suspended_bridge_256x256_0.075                                             |                                                                                     |                                                                                     |                                                                                     |                                                                                     |                                                                                      |                                                                                       |                                                                                       |
| 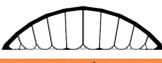   | 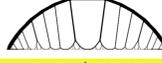   | 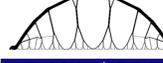   | 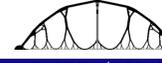   | 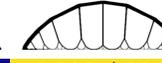   | 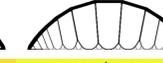   | 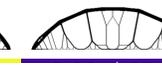   | 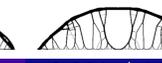   |
| 0.028 / 34.3                                                                        | 0.0 / 33.3                                                                          | 0.131 / 37.7                                                                        | 0.457 / 48.6                                                                        | 0.006 / 32.5                                                                        | 0.0 / 32.3                                                                           | 0.09 / 35.3                                                                           | 0.291 / 41.8                                                                          |
| anchored_suspended_bridge_64x64_0.15                                                |                                                                                     |                                                                                     |                                                                                     |                                                                                     |                                                                                      |                                                                                       |                                                                                       |
| 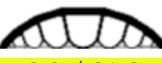   | 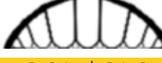   | 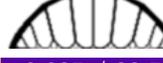   | 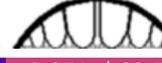   | 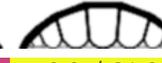   | 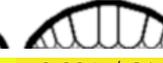   | 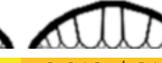   | 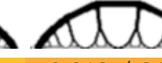   |
| 0.0 / 21.6                                                                          | 0.01 / 21.9                                                                         | 0.085 / 23.5                                                                        | 0.051 / 22.7                                                                        | 0.0 / 21.0                                                                          | 0.004 / 21.1                                                                         | 0.013 / 21.3                                                                          | 0.018 / 21.4                                                                          |
| cantilever_beam_full_192x64_0.3                                                     |                                                                                     |                                                                                     |                                                                                     |                                                                                     |                                                                                      |                                                                                       |                                                                                       |
| 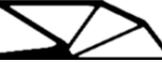 | 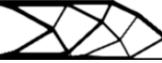 | 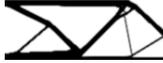 | 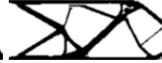 | 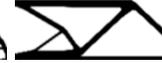 | 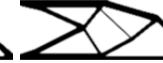 | 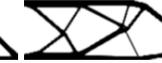 | 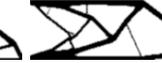 |
| 0.0 / 311.8                                                                         | 0.002 / 312.4                                                                       | 0.01 / 314.9                                                                        | 0.259 / 392.7                                                                       | 0.0 / 305.2                                                                         | 0.004 / 306.5                                                                        | 0.03 / 314.5                                                                          | 0.064 / 324.9                                                                         |
| cantilever_beam_full_384x128_0.15                                                   |                                                                                     |                                                                                     |                                                                                     |                                                                                     |                                                                                      |                                                                                       |                                                                                       |
| 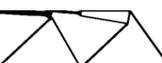 | 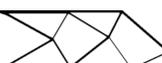 | 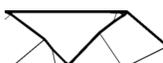 | 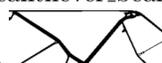 | 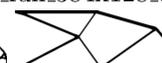 | 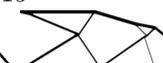 | 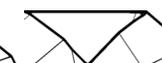 | 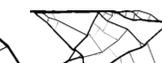 |
| 0.065 / 639.3                                                                       | 0.0 / 600.4                                                                         | 0.055 / 633.4                                                                       | 0.978 / 1187.7                                                                      | 0.0 / 586.7                                                                         | 0.023 / 600.2                                                                        | 0.08 / 633.4                                                                          | 0.373 / 805.5                                                                         |
| cantilever_beam_full_384x128_0.2                                                    |                                                                                     |                                                                                     |                                                                                     |                                                                                     |                                                                                      |                                                                                       |                                                                                       |
| 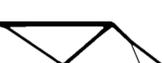 | 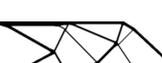 | 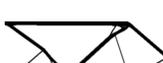 | 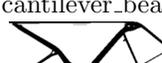 | 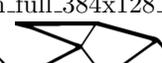 | 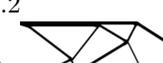 | 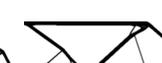 | 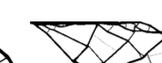 |
| 0.017 / 445.5                                                                       | 0.0 / 437.9                                                                         | 0.035 / 453.1                                                                       | 0.701 / 744.7                                                                       | 0.0 / 426.7                                                                         | 0.022 / 435.9                                                                        | 0.062 / 453.1                                                                         | 0.23 / 524.7                                                                          |
| cantilever_beam_full_96x32_0.4                                                      |                                                                                     |                                                                                     |                                                                                     |                                                                                     |                                                                                      |                                                                                       |                                                                                       |
| 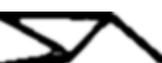 | 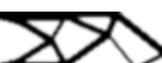 | 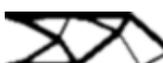 | 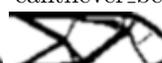 | 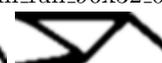 | 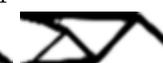 | 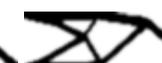 | 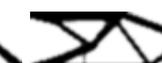 |
| 0.0 / 250.8                                                                         | 0.019 / 255.5                                                                       | 0.023 / 256.7                                                                       | 0.126 / 282.4                                                                       | 0.0 / 247.3                                                                         | 0.005 / 248.6                                                                        | 0.013 / 250.5                                                                         | 0.031 / 255.0                                                                         |
| cantilever_beam_two_point_128x96_0.3                                                |                                                                                     |                                                                                     |                                                                                     |                                                                                     |                                                                                      |                                                                                       |                                                                                       |
| 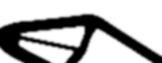 | 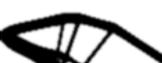 | 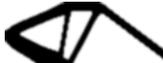 | 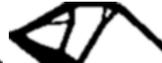 | 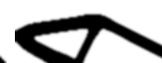 | 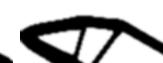 | 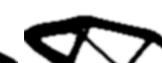 | 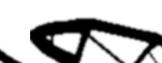 |
| 0.0 / 111.0                                                                         | 0.002 / 111.2                                                                       | 0.044 / 115.9                                                                       | 0.124 / 124.9                                                                       | 0.0 / 109.1                                                                         | 0.002 / 109.3                                                                        | 0.026 / 111.9                                                                         | 0.04 / 113.4                                                                          |

| Typical sample                                                                     |                                                                                     |                                                                                     |                                                                                     | Best of ensemble                                                                     |                                                                                       |                                                                                       |                                                                                       |
|------------------------------------------------------------------------------------|-------------------------------------------------------------------------------------|-------------------------------------------------------------------------------------|-------------------------------------------------------------------------------------|--------------------------------------------------------------------------------------|---------------------------------------------------------------------------------------|---------------------------------------------------------------------------------------|---------------------------------------------------------------------------------------|
| CNN-LBFGS                                                                          | MMA                                                                                 | OC                                                                                  | Pixel-LBFGS                                                                         | CNN-LBFGS                                                                            | MMA                                                                                   | OC                                                                                    | Pixel-LBFGS                                                                           |
| cantilever_beam_two_point_256x192_0.15                                             |                                                                                     |                                                                                     |                                                                                     |                                                                                      |                                                                                       |                                                                                       |                                                                                       |
| 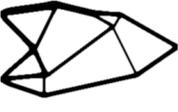   | 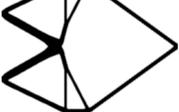   | 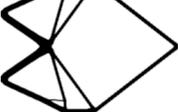   | 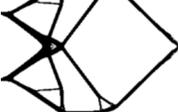   | 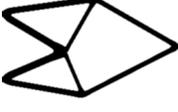   | 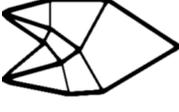   | 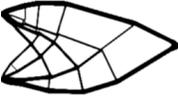   | 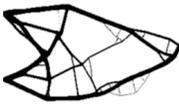   |
| 0.0 / 216.4                                                                        | 0.045 / 226.3                                                                       | 0.092 / 236.3                                                                       | 0.315 / 284.6                                                                       | 0.0 / 205.6                                                                          | 0.015 / 208.7                                                                         | 0.095 / 225.2                                                                         | 0.185 / 243.7                                                                         |
| cantilever_beam_two_point_256x192_0.2                                              |                                                                                     |                                                                                     |                                                                                     |                                                                                      |                                                                                       |                                                                                       |                                                                                       |
| 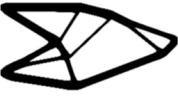   | 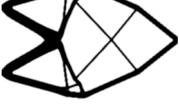   | 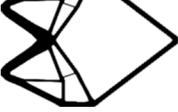   | 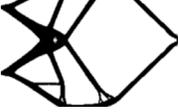   | 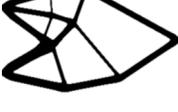   | 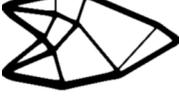   | 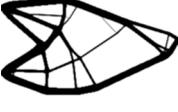   | 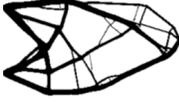   |
| 0.0 / 159.6                                                                        | 0.026 / 163.8                                                                       | 0.072 / 171.0                                                                       | 0.28 / 204.4                                                                        | 0.0 / 155.8                                                                          | 0.003 / 156.3                                                                         | 0.057 / 164.6                                                                         | 0.135 / 176.8                                                                         |
| cantilever_beam_two_point_64x48_0.4                                                |                                                                                     |                                                                                     |                                                                                     |                                                                                      |                                                                                       |                                                                                       |                                                                                       |
| 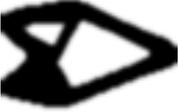   | 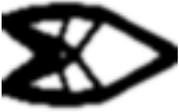   | 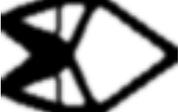   | 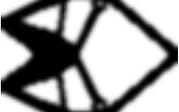   | 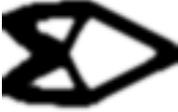   | 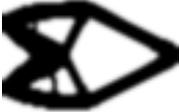   | 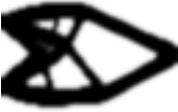   | 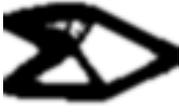   |
| 0.005 / 85.7                                                                       | 0.0 / 85.3                                                                          | 0.046 / 89.2                                                                        | 0.075 / 91.7                                                                        | 0.0 / 84.8                                                                           | 0.001 / 85.0                                                                          | 0.004 / 85.1                                                                          | 0.019 / 86.4                                                                          |
| canyon_bridge_128x128_0.12                                                         |                                                                                     |                                                                                     |                                                                                     |                                                                                      |                                                                                       |                                                                                       |                                                                                       |
| 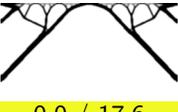   | 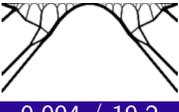   | 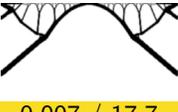   | 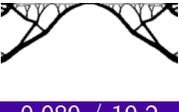   | 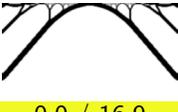   | 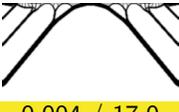   | 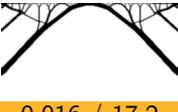   | 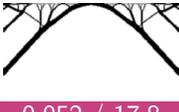   |
| 0.0 / 17.6                                                                         | 0.094 / 19.2                                                                        | 0.007 / 17.7                                                                        | 0.089 / 19.2                                                                        | 0.0 / 16.9                                                                           | 0.004 / 17.0                                                                          | 0.016 / 17.2                                                                          | 0.052 / 17.8                                                                          |
| canyon_bridge_256x256_0.05                                                         |                                                                                     |                                                                                     |                                                                                     |                                                                                      |                                                                                       |                                                                                       |                                                                                       |
| 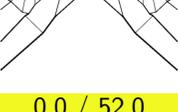 | 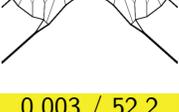 | 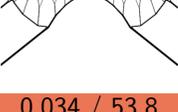 | 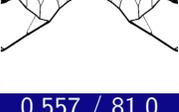 | 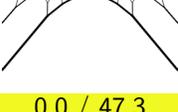 | 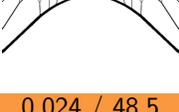 | 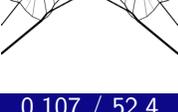 | 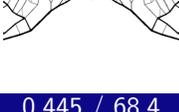 |
| 0.0 / 52.0                                                                         | 0.003 / 52.2                                                                        | 0.034 / 53.8                                                                        | 0.557 / 81.0                                                                        | 0.0 / 47.3                                                                           | 0.024 / 48.5                                                                          | 0.107 / 52.4                                                                          | 0.445 / 68.4                                                                          |
| canyon_bridge_256x256_0.1                                                          |                                                                                     |                                                                                     |                                                                                     |                                                                                      |                                                                                       |                                                                                       |                                                                                       |
| 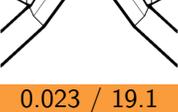 | 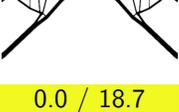 | 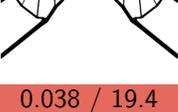 | 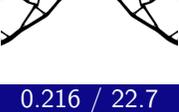 | 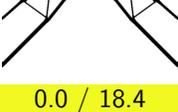 | 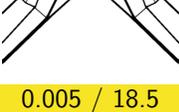 | 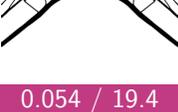 | 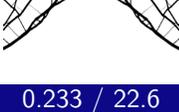 |
| 0.023 / 19.1                                                                       | 0.0 / 18.7                                                                          | 0.038 / 19.4                                                                        | 0.216 / 22.7                                                                        | 0.0 / 18.4                                                                           | 0.005 / 18.5                                                                          | 0.054 / 19.4                                                                          | 0.233 / 22.6                                                                          |
| canyon_bridge_64x64_0.16                                                           |                                                                                     |                                                                                     |                                                                                     |                                                                                      |                                                                                       |                                                                                       |                                                                                       |
| 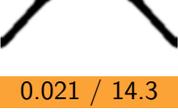 | 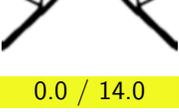 | 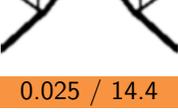 | 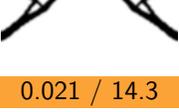 | 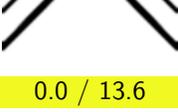 | 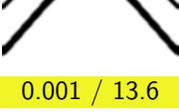 | 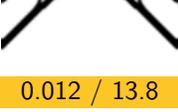 | 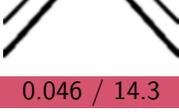 |
| 0.021 / 14.3                                                                       | 0.0 / 14.0                                                                          | 0.025 / 14.4                                                                        | 0.021 / 14.3                                                                        | 0.0 / 13.6                                                                           | 0.001 / 13.6                                                                          | 0.012 / 13.8                                                                          | 0.046 / 14.3                                                                          |
| causeway_bridge_low_128x128_0.1                                                    |                                                                                     |                                                                                     |                                                                                     |                                                                                      |                                                                                       |                                                                                       |                                                                                       |
| 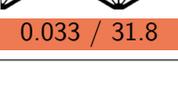 | 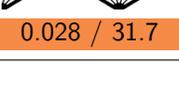 | 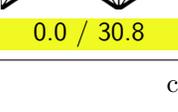 | 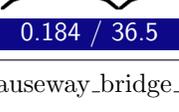 | 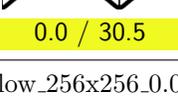 | 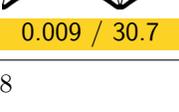 | 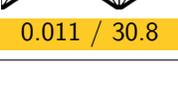 | 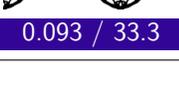 |
| 0.033 / 31.8                                                                       | 0.028 / 31.7                                                                        | 0.0 / 30.8                                                                          | 0.184 / 36.5                                                                        | 0.0 / 30.5                                                                           | 0.009 / 30.7                                                                          | 0.011 / 30.8                                                                          | 0.093 / 33.3                                                                          |
| causeway_bridge_low_256x256_0.08                                                   |                                                                                     |                                                                                     |                                                                                     |                                                                                      |                                                                                       |                                                                                       |                                                                                       |
| 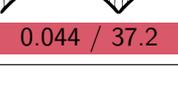 | 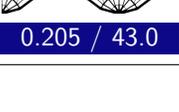 | 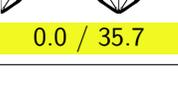 | 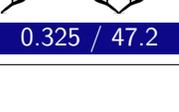 | 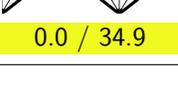 | 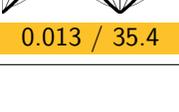 | 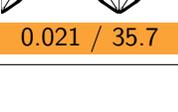 | 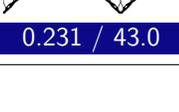 |
| 0.044 / 37.2                                                                       | 0.205 / 43.0                                                                        | 0.0 / 35.7                                                                          | 0.325 / 47.2                                                                        | 0.0 / 34.9                                                                           | 0.013 / 35.4                                                                          | 0.021 / 35.7                                                                          | 0.231 / 43.0                                                                          |

| Typical sample                      |               |               |               | Best of ensemble |               |               |               |
|-------------------------------------|---------------|---------------|---------------|------------------|---------------|---------------|---------------|
| CNN-LBFGS                           | MMA           | OC            | Pixel-LBFGS   | CNN-LBFGS        | MMA           | OC            | Pixel-LBFGS   |
| causeway_bridge_low_64x64_0.12      |               |               |               |                  |               |               |               |
|                                     |               |               |               |                  |               |               |               |
| 0.029 / 29.4                        | 0.015 / 29.0  | 0.0 / 28.6    | 0.115 / 31.9  | 0.006 / 28.8     | 0.003 / 28.7  | 0.0 / 28.6    | 0.027 / 29.4  |
| causeway_bridge_middle_128x128_0.1  |               |               |               |                  |               |               |               |
|                                     |               |               |               |                  |               |               |               |
| 0.02 / 29.6                         | 0.029 / 29.8  | 0.0 / 29.0    | 0.129 / 32.7  | 0.0 / 28.4       | 0.005 / 28.6  | 0.019 / 29.0  | 0.151 / 32.7  |
| causeway_bridge_middle_256x256_0.08 |               |               |               |                  |               |               |               |
|                                     |               |               |               |                  |               |               |               |
| 0.013 / 34.3                        | 0.123 / 38.0  | 0.0 / 33.8    | 0.271 / 43.0  | 0.003 / 32.7     | 0.0 / 32.6    | 0.019 / 33.2  | 0.118 / 36.5  |
| causeway_bridge_middle_64x64_0.12   |               |               |               |                  |               |               |               |
|                                     |               |               |               |                  |               |               |               |
| 0.013 / 27.4                        | 0.029 / 27.8  | 0.0 / 27.0    | 0.077 / 29.1  | 0.001 / 26.7     | 0.002 / 26.7  | 0.0 / 26.6    | 0.033 / 27.5  |
| causeway_bridge_top_128x128_0.2     |               |               |               |                  |               |               |               |
|                                     |               |               |               |                  |               |               |               |
| 0.021 / 17.7                        | 0.0 / 17.4    | 0.033 / 17.9  | 0.07 / 18.6   | 0.01 / 17.4      | 0.0 / 17.3    | 0.014 / 17.5  | 0.076 / 18.6  |
| causeway_bridge_top_128x64_0.3      |               |               |               |                  |               |               |               |
|                                     |               |               |               |                  |               |               |               |
| 0.007 / 21.1                        | 0.0 / 20.9    | 0.001 / 20.9  | 0.043 / 21.8  | 0.001 / 20.8     | 0.0 / 20.8    | 0.007 / 20.9  | 0.03 / 21.4   |
| causeway_bridge_top_256x128_0.2     |               |               |               |                  |               |               |               |
|                                     |               |               |               |                  |               |               |               |
| 0.0 / 30.0                          | 0.016 / 30.5  | 0.005 / 30.2  | 0.11 / 33.3   | 0.006 / 29.4     | 0.0 / 29.2    | 0.034 / 30.2  | 0.13 / 33.0   |
| causeway_bridge_top_256x256_0.1     |               |               |               |                  |               |               |               |
|                                     |               |               |               |                  |               |               |               |
| 0.0 / 34.5                          | 0.08 / 37.2   | 0.017 / 35.1  | 0.203 / 41.4  | 0.0 / 32.8       | 0.001 / 32.9  | 0.067 / 35.0  | 0.262 / 41.4  |
| causeway_bridge_top_64x64_0.3       |               |               |               |                  |               |               |               |
|                                     |               |               |               |                  |               |               |               |
| 0.009 / 12.7                        | 0.004 / 12.6  | 0.0 / 12.6    | 0.027 / 12.9  | 0.002 / 12.5     | 0.0 / 12.5    | 0.001 / 12.5  | 0.016 / 12.7  |
| center_support_128x128_0.1          |               |               |               |                  |               |               |               |
|                                     |               |               |               |                  |               |               |               |
| 0.0 / 54.8                          | 0.048 / 57.4  | 0.055 / 57.8  | 0.208 / 66.2  | 0.0 / 51.4       | 0.007 / 51.8  | 0.058 / 54.4  | 0.165 / 59.9  |
| center_support_256x256_0.05         |               |               |               |                  |               |               |               |
|                                     |               |               |               |                  |               |               |               |
| 0.0 / 125.6                         | 0.074 / 134.9 | 0.074 / 134.9 | 0.497 / 188.0 | 0.0 / 108.3      | 0.068 / 115.7 | 0.245 / 134.9 | 0.655 / 179.3 |
| center_support_256x256_0.1          |               |               |               |                  |               |               |               |
|                                     |               |               |               |                  |               |               |               |
| 0.0 / 44.1                          | 0.056 / 46.5  | 0.052 / 46.3  | 0.286 / 56.6  | 0.0 / 41.9       | 0.011 / 42.3  | 0.086 / 45.5  | 0.287 / 53.9  |

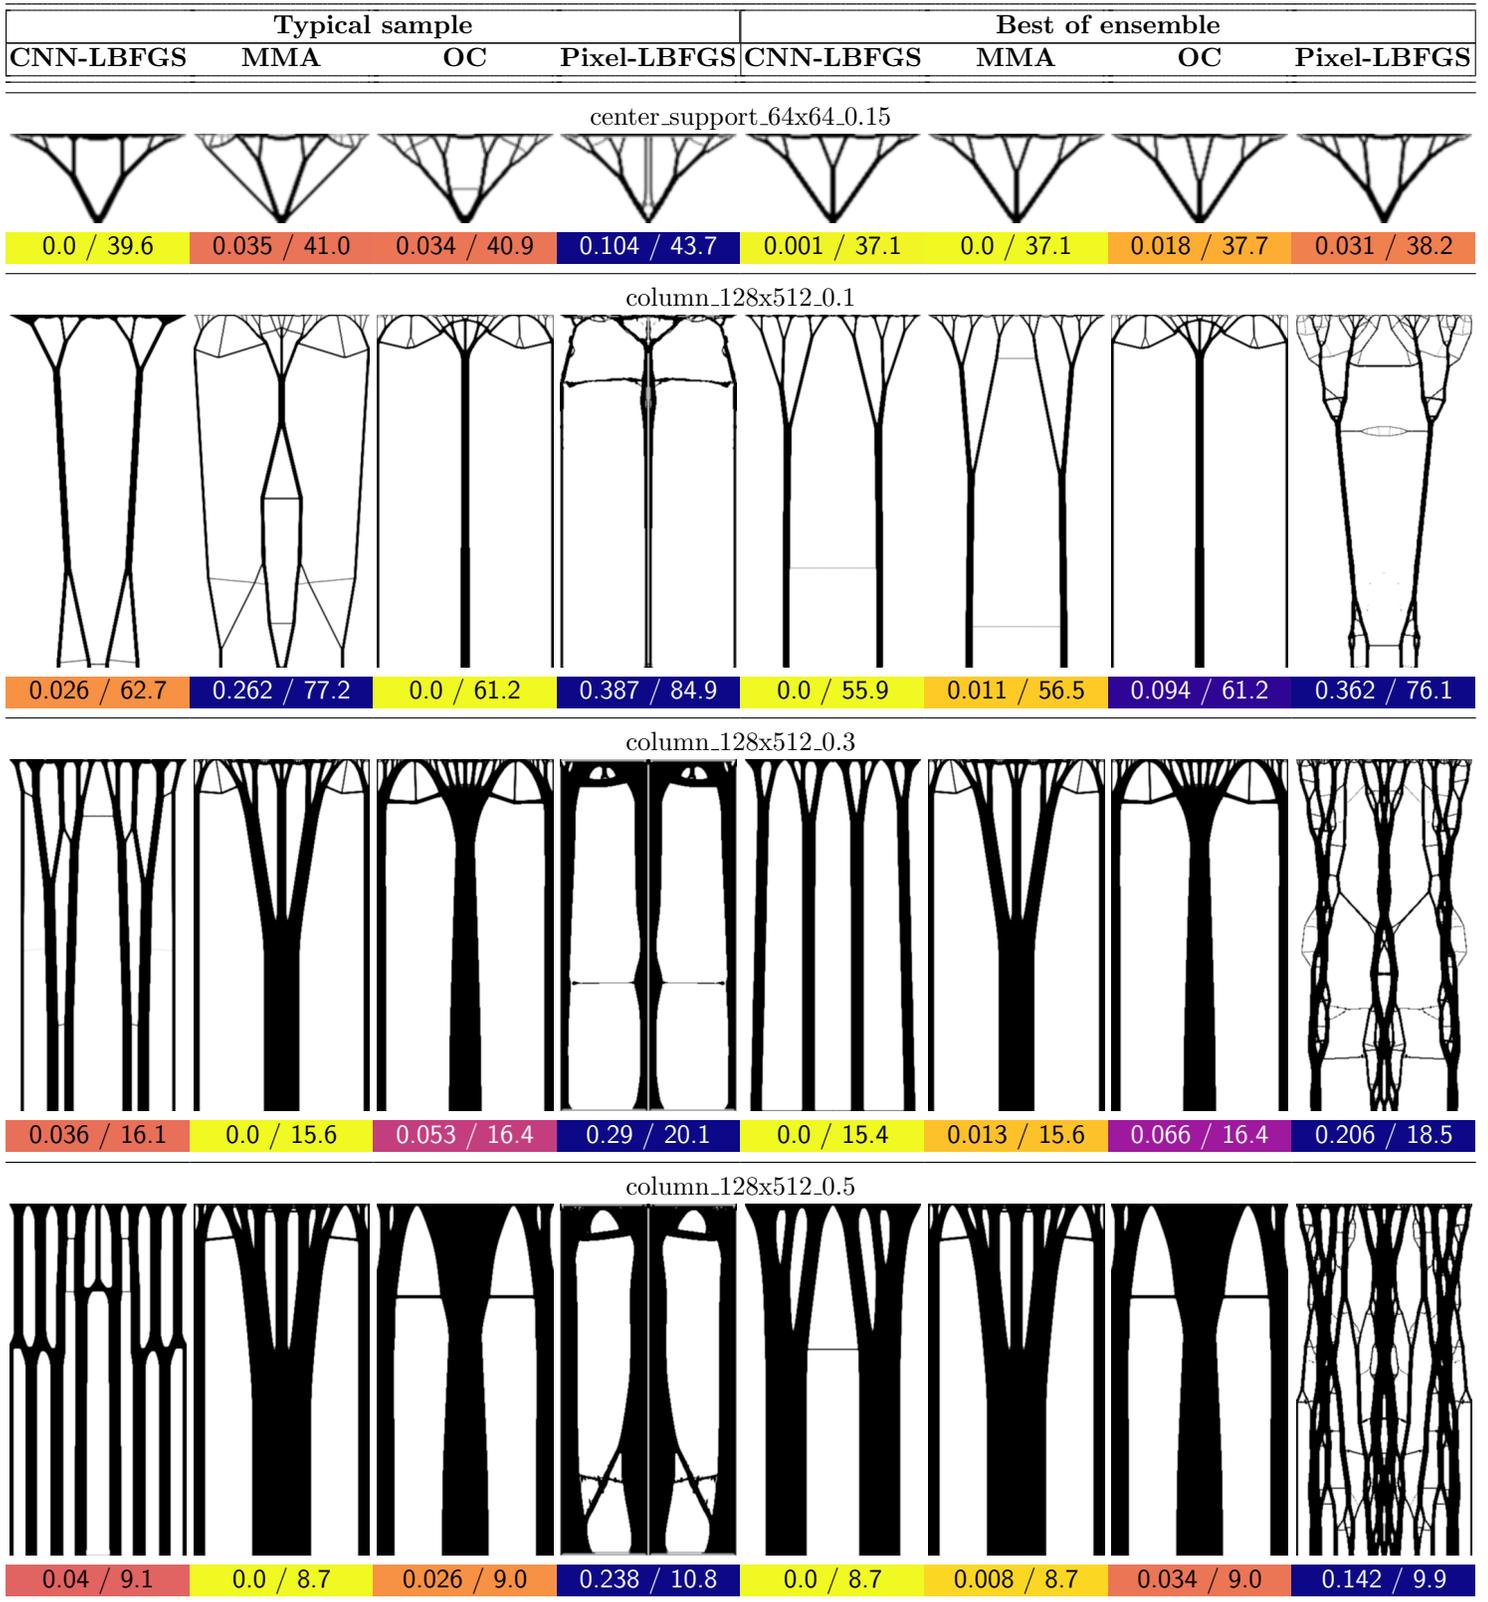

| Typical sample                                                                     |                                                                                     |                                                                                     |                                                                                     | Best of ensemble                                                                     |                                                                                       |                                                                                       |                                                                                       |
|------------------------------------------------------------------------------------|-------------------------------------------------------------------------------------|-------------------------------------------------------------------------------------|-------------------------------------------------------------------------------------|--------------------------------------------------------------------------------------|---------------------------------------------------------------------------------------|---------------------------------------------------------------------------------------|---------------------------------------------------------------------------------------|
| CNN-LBFGS                                                                          | MMA                                                                                 | OC                                                                                  | Pixel-LBFGS                                                                         | CNN-LBFGS                                                                            | MMA                                                                                   | OC                                                                                    | Pixel-LBFGS                                                                           |
| column_32x128_0.3                                                                  |                                                                                     |                                                                                     |                                                                                     |                                                                                      |                                                                                       |                                                                                       |                                                                                       |
| 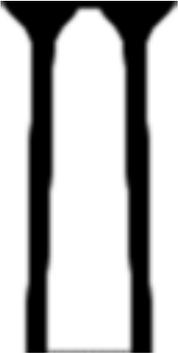   | 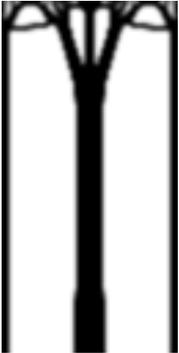   | 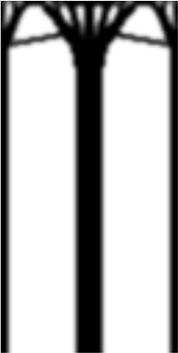   | 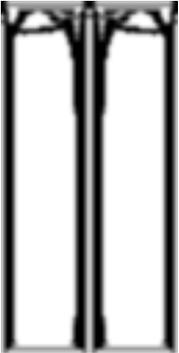   | 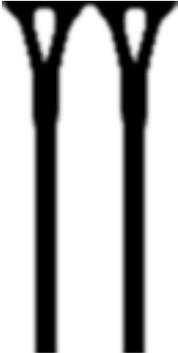   | 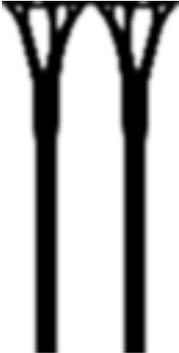   | 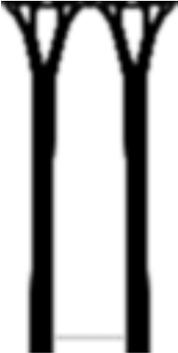   | 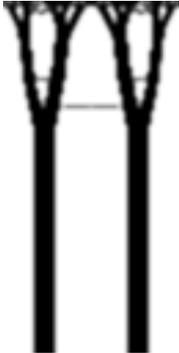   |
| 0.012 / 19.7                                                                       | 0.0 / 19.5                                                                          | 0.009 / 19.6                                                                        | 0.295 / 25.2                                                                        | 0.003 / 18.8                                                                         | 0.0 / 18.8                                                                            | 0.005 / 18.9                                                                          | 0.026 / 19.3                                                                          |
| column_64x256_0.3                                                                  |                                                                                     |                                                                                     |                                                                                     |                                                                                      |                                                                                       |                                                                                       |                                                                                       |
| 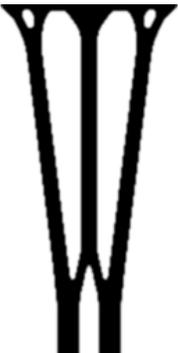   | 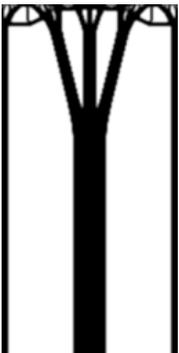   | 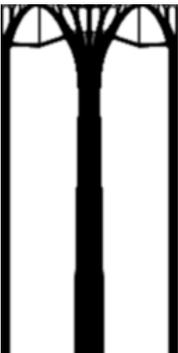   | 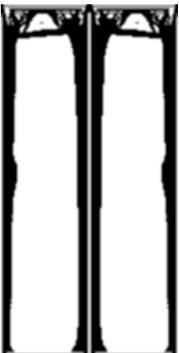   | 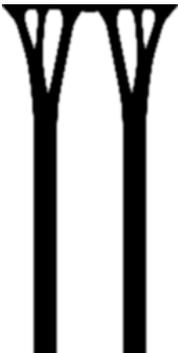   | 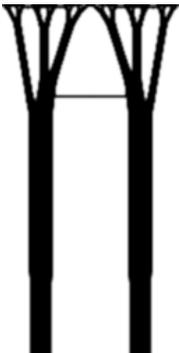   | 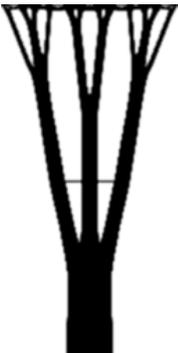   | 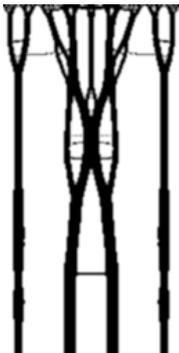   |
| 0.017 / 17.2                                                                       | 0.0 / 16.9                                                                          | 0.024 / 17.3                                                                        | 0.264 / 21.4                                                                        | 0.0 / 16.4                                                                           | 0.014 / 16.6                                                                          | 0.047 / 17.2                                                                          | 0.146 / 18.8                                                                          |
| crane_128x128_0.2                                                                  |                                                                                     |                                                                                     |                                                                                     |                                                                                      |                                                                                       |                                                                                       |                                                                                       |
| 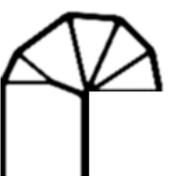 | 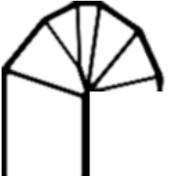 | 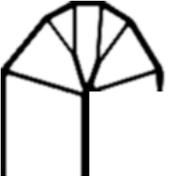 | 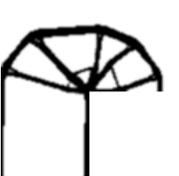 | 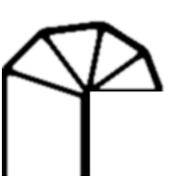 | 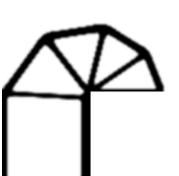 | 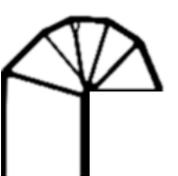 | 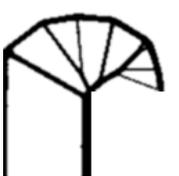 |
| 0.0 / 140.9                                                                        | 0.034 / 145.6                                                                       | 0.033 / 145.4                                                                       | 0.252 / 176.4                                                                       | 0.0 / 135.9                                                                          | 0.008 / 137.0                                                                         | 0.023 / 139.0                                                                         | 0.102 / 149.8                                                                         |
| crane_256x256_0.1                                                                  |                                                                                     |                                                                                     |                                                                                     |                                                                                      |                                                                                       |                                                                                       |                                                                                       |
| 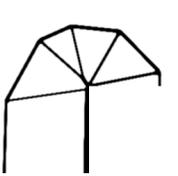 | 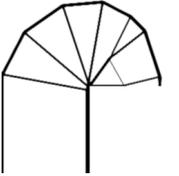 | 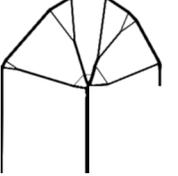 | 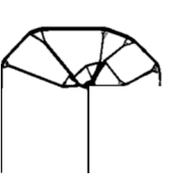 | 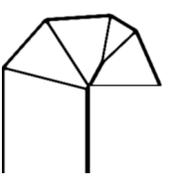 | 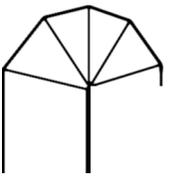 | 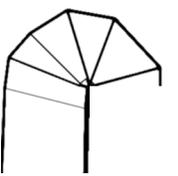 | 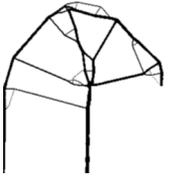 |
| 0.0 / 293.2                                                                        | 0.019 / 298.7                                                                       | 0.032 / 302.5                                                                       | 0.456 / 426.8                                                                       | 0.0 / 276.1                                                                          | 0.003 / 277.0                                                                         | 0.096 / 302.5                                                                         | 0.322 / 364.9                                                                         |
| crane_256x256_0.15                                                                 |                                                                                     |                                                                                     |                                                                                     |                                                                                      |                                                                                       |                                                                                       |                                                                                       |
| 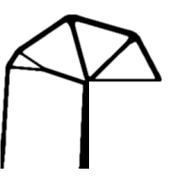 | 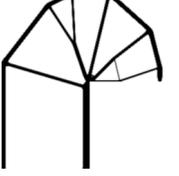 | 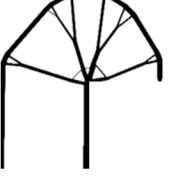 | 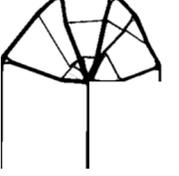 | 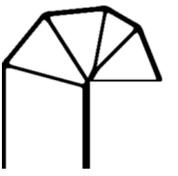 | 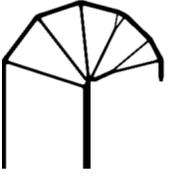 | 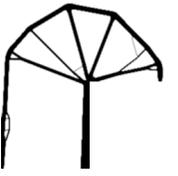 | 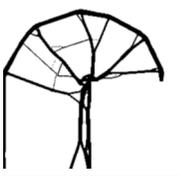 |
| 0.0 / 175.0                                                                        | 0.01 / 176.8                                                                        | 0.05 / 183.7                                                                        | 0.558 / 272.6                                                                       | 0.0 / 170.0                                                                          | 0.005 / 170.9                                                                         | 0.046 / 177.8                                                                         | 0.242 / 211.2                                                                         |

| Typical sample                                                                     |                                                                                     |                                                                                     |                                                                                     | Best of ensemble                                                                    |                                                                                       |                                                                                       |                                                                                       |
|------------------------------------------------------------------------------------|-------------------------------------------------------------------------------------|-------------------------------------------------------------------------------------|-------------------------------------------------------------------------------------|-------------------------------------------------------------------------------------|---------------------------------------------------------------------------------------|---------------------------------------------------------------------------------------|---------------------------------------------------------------------------------------|
| CNN-LBFGS                                                                          | MMA                                                                                 | OC                                                                                  | Pixel-LBFGS                                                                         | CNN-LBFGS                                                                           | MMA                                                                                   | OC                                                                                    | Pixel-LBFGS                                                                           |
| crane_64x64_0.3                                                                    |                                                                                     |                                                                                     |                                                                                     |                                                                                     |                                                                                       |                                                                                       |                                                                                       |
| 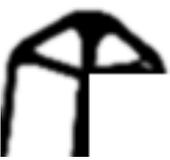   | 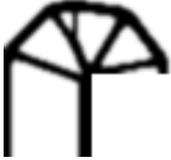   | 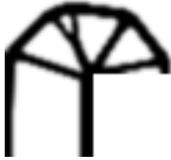   | 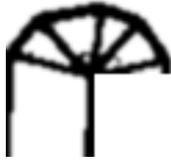   | 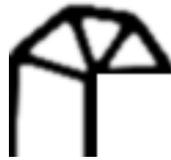   | 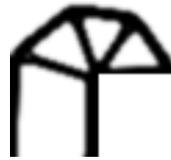   | 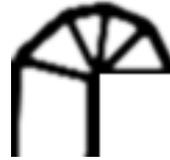   | 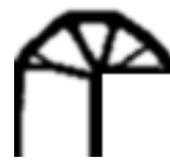   |
| 0.038 / 102.1                                                                      | 0.001 / 98.5                                                                        | 0.0 / 98.4                                                                          | 0.114 / 109.7                                                                       | 0.0 / 97.3                                                                          | 0.0 / 97.3                                                                            | 0.004 / 97.7                                                                          | 0.019 / 99.1                                                                          |
| dam_128x128_0.15                                                                   |                                                                                     |                                                                                     |                                                                                     |                                                                                     |                                                                                       |                                                                                       |                                                                                       |
| 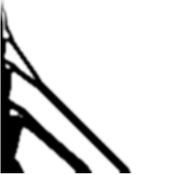   | 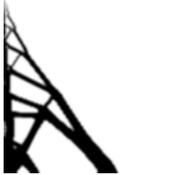   | 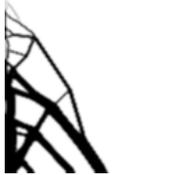   | 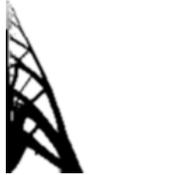   | 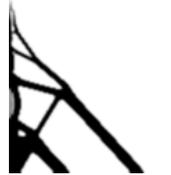   | 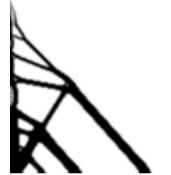   | 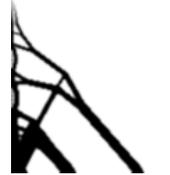   | 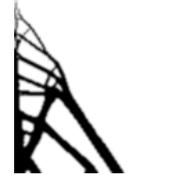   |
| 0.034 / 7.8                                                                        | 0.0 / 7.6                                                                           | 0.071 / 8.1                                                                         | 0.31 / 9.9                                                                          | 0.007 / 7.2                                                                         | 0.0 / 7.2                                                                             | 0.011 / 7.2                                                                           | 0.119 / 8.0                                                                           |
| dam_256x256_0.05                                                                   |                                                                                     |                                                                                     |                                                                                     |                                                                                     |                                                                                       |                                                                                       |                                                                                       |
| 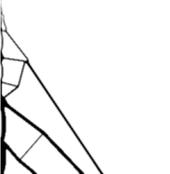   | 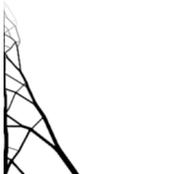   | 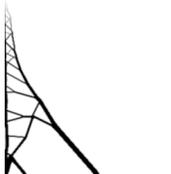   | 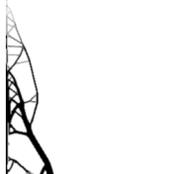   | 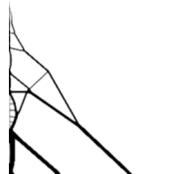   | 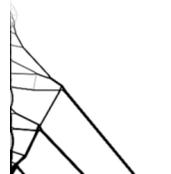   | 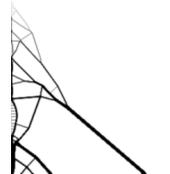   | 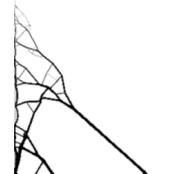   |
| 0.0 / 33.4                                                                         | 0.117 / 37.3                                                                        | 0.01 / 33.7                                                                         | 1.779 / 92.8                                                                        | 0.024 / 30.6                                                                        | 0.0 / 29.9                                                                            | 0.07 / 32.0                                                                           | 0.236 / 37.0                                                                          |
| dam_256x256_0.1                                                                    |                                                                                     |                                                                                     |                                                                                     |                                                                                     |                                                                                       |                                                                                       |                                                                                       |
| 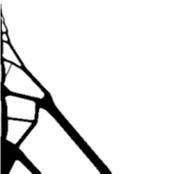 | 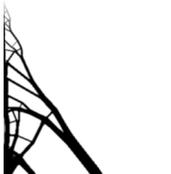 | 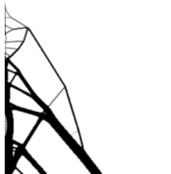 | 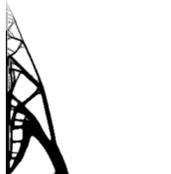 | 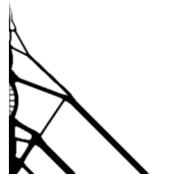 | 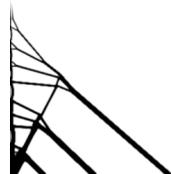 | 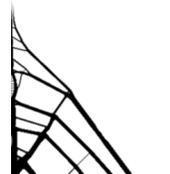 | 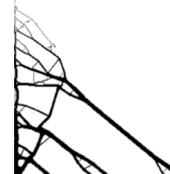 |
| 0.0 / 11.6                                                                         | 0.043 / 12.1                                                                        | 0.058 / 12.3                                                                        | 0.638 / 19.0                                                                        | 0.013 / 10.7                                                                        | 0.0 / 10.6                                                                            | 0.062 / 11.2                                                                          | 0.215 / 12.9                                                                          |
| dam_256x256_0.2                                                                    |                                                                                     |                                                                                     |                                                                                     |                                                                                     |                                                                                       |                                                                                       |                                                                                       |
| 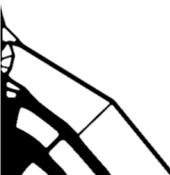 | 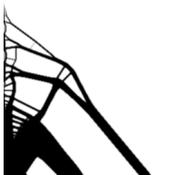 | 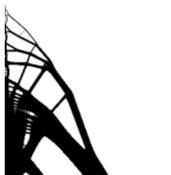 | 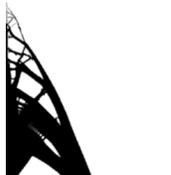 | 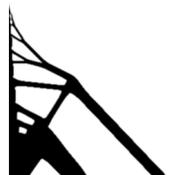 | 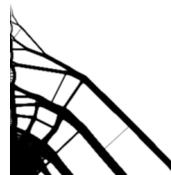 | 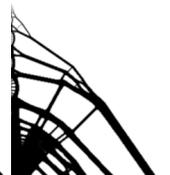 | 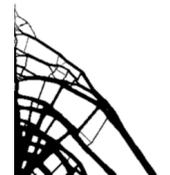 |
| 0.028 / 4.6                                                                        | 0.0 / 4.4                                                                           | 0.113 / 5.0                                                                         | 0.287 / 5.7                                                                         | 0.0 / 4.4                                                                           | 0.004 / 4.4                                                                           | 0.029 / 4.5                                                                           | 0.135 / 5.0                                                                           |
| dam_64x64_0.2                                                                      |                                                                                     |                                                                                     |                                                                                     |                                                                                     |                                                                                       |                                                                                       |                                                                                       |
| 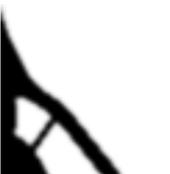 | 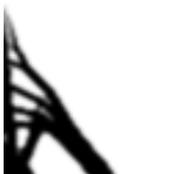 | 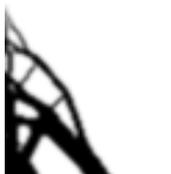 | 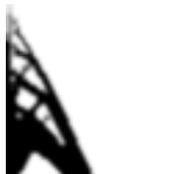 | 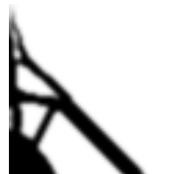 | 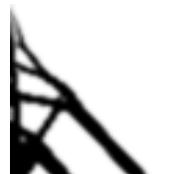 | 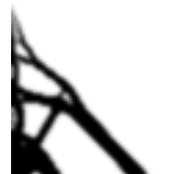 | 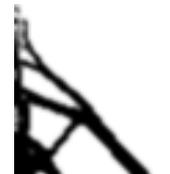 |
| 0.031 / 6.3                                                                        | 0.0 / 6.1                                                                           | 0.037 / 6.3                                                                         | 0.146 / 7.0                                                                         | 0.009 / 5.8                                                                         | 0.0 / 5.8                                                                             | 0.006 / 5.8                                                                           | 0.033 / 6.0                                                                           |

| Typical sample                                                                     |                                                                                     |                                                                                     |                                                                                     | Best of ensemble                                                                     |                                                                                       |                                                                                       |                                                                                       |
|------------------------------------------------------------------------------------|-------------------------------------------------------------------------------------|-------------------------------------------------------------------------------------|-------------------------------------------------------------------------------------|--------------------------------------------------------------------------------------|---------------------------------------------------------------------------------------|---------------------------------------------------------------------------------------|---------------------------------------------------------------------------------------|
| CNN-LBFGS                                                                          | MMA                                                                                 | OC                                                                                  | Pixel-LBFGS                                                                         | CNN-LBFGS                                                                            | MMA                                                                                   | OC                                                                                    | Pixel-LBFGS                                                                           |
| drawbridge_128x128_0.15                                                            |                                                                                     |                                                                                     |                                                                                     |                                                                                      |                                                                                       |                                                                                       |                                                                                       |
| 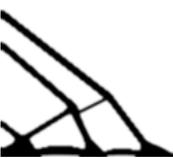   | 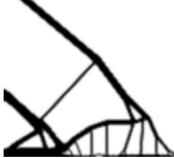   | 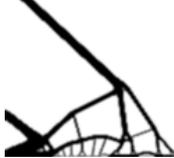   | 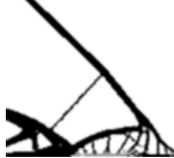   | 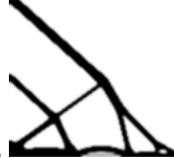   | 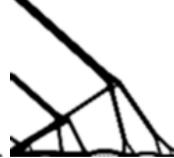   | 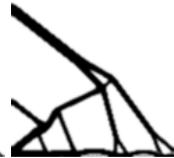   | 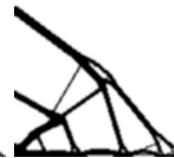   |
| 0.014 / 18.2                                                                       | 0.004 / 18.0                                                                        | 0.0 / 17.9                                                                          | 0.24 / 22.2                                                                         | 0.02 / 16.9                                                                          | 0.0 / 16.6                                                                            | 0.038 / 17.3                                                                          | 0.093 / 18.2                                                                          |
| drawbridge_256x256_0.1                                                             |                                                                                     |                                                                                     |                                                                                     |                                                                                      |                                                                                       |                                                                                       |                                                                                       |
| 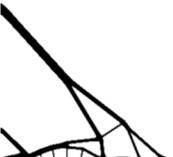   | 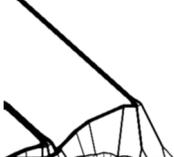   | 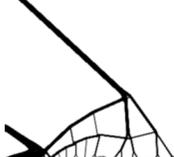   | 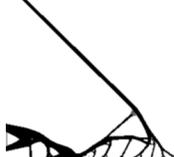   | 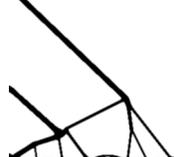   | 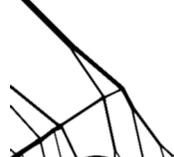   | 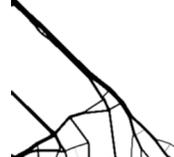   | 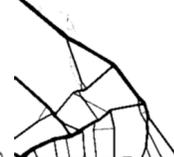   |
| 0.0 / 26.4                                                                         | 0.005 / 26.5                                                                        | 0.049 / 27.7                                                                        | 0.806 / 47.7                                                                        | 0.0 / 24.6                                                                           | 0.0 / 24.6                                                                            | 0.063 / 26.1                                                                          | 0.261 / 31.0                                                                          |
| drawbridge_64x64_0.2                                                               |                                                                                     |                                                                                     |                                                                                     |                                                                                      |                                                                                       |                                                                                       |                                                                                       |
| 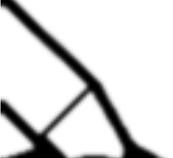   | 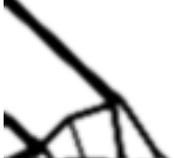   | 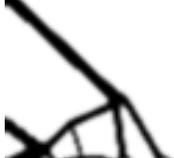   | 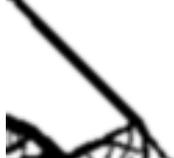   | 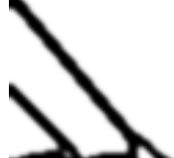   | 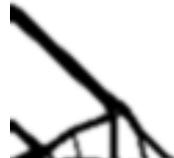   | 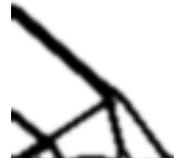   | 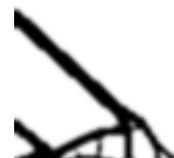   |
| 0.059 / 14.7                                                                       | 0.0 / 13.9                                                                          | 0.008 / 14.0                                                                        | 0.168 / 16.2                                                                        | 0.026 / 13.9                                                                         | 0.0 / 13.6                                                                            | 0.011 / 13.7                                                                          | 0.023 / 13.9                                                                          |
| free_suspended_bridge_128x128_0.1                                                  |                                                                                     |                                                                                     |                                                                                     |                                                                                      |                                                                                       |                                                                                       |                                                                                       |
| 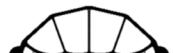 | 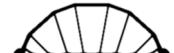 | 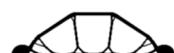 | 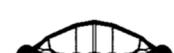 | 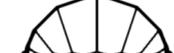 | 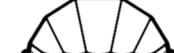 | 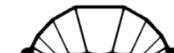 | 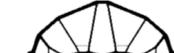 |
| 0.041 / 25.5                                                                       | 0.0 / 24.5                                                                          | 0.137 / 27.9                                                                        | 0.819 / 44.6                                                                        | 0.0 / 24.0                                                                           | 0.005 / 24.1                                                                          | 0.028 / 24.7                                                                          | 0.134 / 27.2                                                                          |
| free_suspended_bridge_256x256_0.05                                                 |                                                                                     |                                                                                     |                                                                                     |                                                                                      |                                                                                       |                                                                                       |                                                                                       |
| 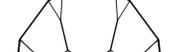 | 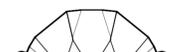 | 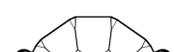 | 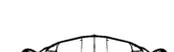 | 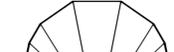 | 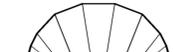 | 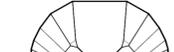 | 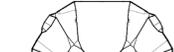 |
| 0.0 / 56.1                                                                         | 0.042 / 58.4                                                                        | 0.183 / 66.3                                                                        | 2.061 / 171.6                                                                       | 0.0 / 49.9                                                                           | 0.028 / 51.3                                                                          | 0.25 / 62.5                                                                           | 0.482 / 74.0                                                                          |
| free_suspended_bridge_256x256_0.075                                                |                                                                                     |                                                                                     |                                                                                     |                                                                                      |                                                                                       |                                                                                       |                                                                                       |
| 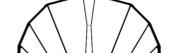 | 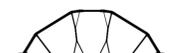 | 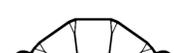 | 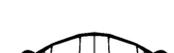 | 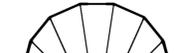 | 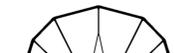 | 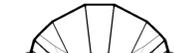 | 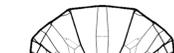 |
| 0.0 / 30.9                                                                         | 0.006 / 31.1                                                                        | 0.182 / 36.5                                                                        | 1.558 / 79.0                                                                        | 0.0 / 28.8                                                                           | 0.02 / 29.4                                                                           | 0.099 / 31.7                                                                          | 0.299 / 37.5                                                                          |
| free_suspended_bridge_64x64_0.15                                                   |                                                                                     |                                                                                     |                                                                                     |                                                                                      |                                                                                       |                                                                                       |                                                                                       |
| 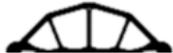 | 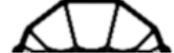 | 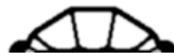 | 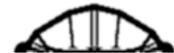 | 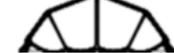 | 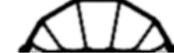 | 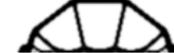 | 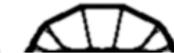 |
| 0.058 / 19.0                                                                       | 0.0 / 17.9                                                                          | 0.073 / 19.3                                                                        | 0.27 / 22.8                                                                         | 0.01 / 18.1                                                                          | 0.0 / 17.9                                                                            | 0.015 / 18.2                                                                          | 0.042 / 18.6                                                                          |
| ground_structure_128x128_0.1                                                       |                                                                                     |                                                                                     |                                                                                     |                                                                                      |                                                                                       |                                                                                       |                                                                                       |
| 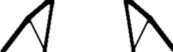 | 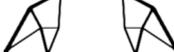 | 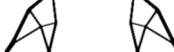 | 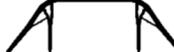 | 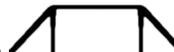 | 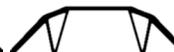 | 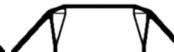 | 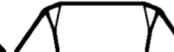 |
| 0.0 / 52.9                                                                         | 0.053 / 55.7                                                                        | 0.064 / 56.3                                                                        | 0.013 / 53.6                                                                        | 0.0 / 49.5                                                                           | 0.006 / 49.8                                                                          | 0.016 / 50.4                                                                          | 0.081 / 53.6                                                                          |

| Typical sample                                                                     |                                                                                     |                                                                                     |                                                                                     | Best of ensemble                                                                     |                                                                                       |                                                                                       |                                                                                       |
|------------------------------------------------------------------------------------|-------------------------------------------------------------------------------------|-------------------------------------------------------------------------------------|-------------------------------------------------------------------------------------|--------------------------------------------------------------------------------------|---------------------------------------------------------------------------------------|---------------------------------------------------------------------------------------|---------------------------------------------------------------------------------------|
| CNN-LBFGS                                                                          | MMA                                                                                 | OC                                                                                  | Pixel-LBFGS                                                                         | CNN-LBFGS                                                                            | MMA                                                                                   | OC                                                                                    | Pixel-LBFGS                                                                           |
| ground_structure_256x256_0.05                                                      |                                                                                     |                                                                                     |                                                                                     |                                                                                      |                                                                                       |                                                                                       |                                                                                       |
| 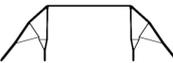   | 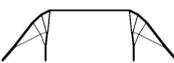   | 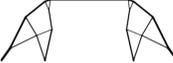   | 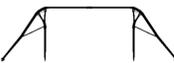   | 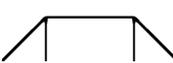   | 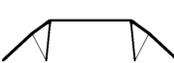   | 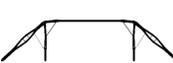   | 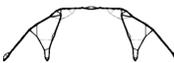   |
| 0.023 / 106.6                                                                      | 0.0 / 104.3                                                                         | 0.089 / 113.5                                                                       | 0.372 / 143.1                                                                       | 0.0 / 97.1                                                                           | 0.027 / 99.7                                                                          | 0.105 / 107.3                                                                         | 0.36 / 132.0                                                                          |
| ground_structure_256x256_0.07                                                      |                                                                                     |                                                                                     |                                                                                     |                                                                                      |                                                                                       |                                                                                       |                                                                                       |
| 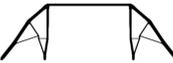   | 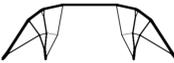   | 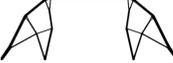   | 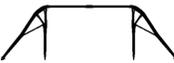   | 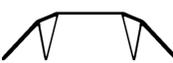   | 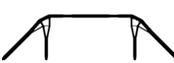   | 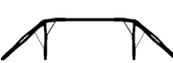   | 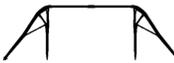   |
| 0.0 / 70.5                                                                         | 0.02 / 71.9                                                                         | 0.042 / 73.5                                                                        | 0.102 / 77.7                                                                        | 0.0 / 66.9                                                                           | 0.013 / 67.7                                                                          | 0.061 / 70.9                                                                          | 0.162 / 77.7                                                                          |
| ground_structure_64x64_0.12                                                        |                                                                                     |                                                                                     |                                                                                     |                                                                                      |                                                                                       |                                                                                       |                                                                                       |
| 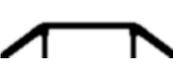   | 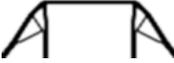   | 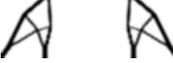   | 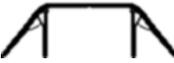   | 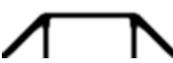   | 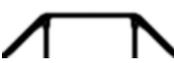   | 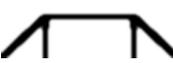   | 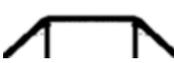   |
| 0.0 / 49.3                                                                         | 0.051 / 51.8                                                                        | 0.213 / 59.8                                                                        | 0.011 / 49.8                                                                        | 0.0 / 44.8                                                                           | 0.0 / 44.8                                                                            | 0.007 / 45.1                                                                          | 0.023 / 45.9                                                                          |
| hoop_128x256_0.15                                                                  |                                                                                     |                                                                                     |                                                                                     |                                                                                      |                                                                                       |                                                                                       |                                                                                       |
| 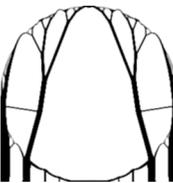   | 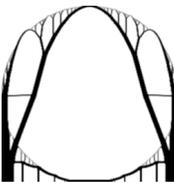   | 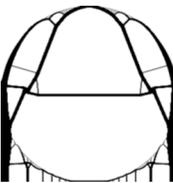   | 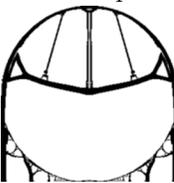   | 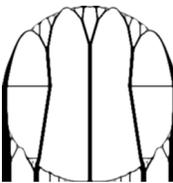   | 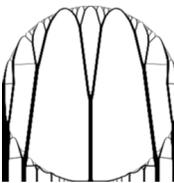   | 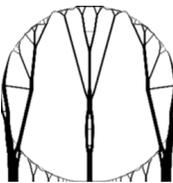   | 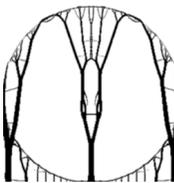   |
| 0.0 / 1.1                                                                          | 0.077 / 1.2                                                                         | 0.25 / 1.4                                                                          | 1.198 / 2.5                                                                         | 0.0 / 1.1                                                                            | 0.012 / 1.1                                                                           | 0.091 / 1.2                                                                           | 0.209 / 1.3                                                                           |
| hoop_32x64_0.25                                                                    |                                                                                     |                                                                                     |                                                                                     |                                                                                      |                                                                                       |                                                                                       |                                                                                       |
| 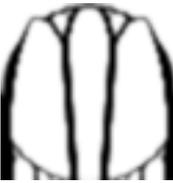 | 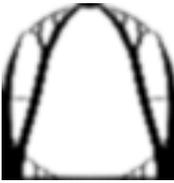 | 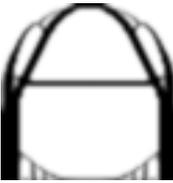 | 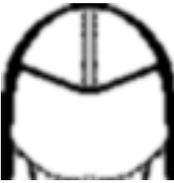 | 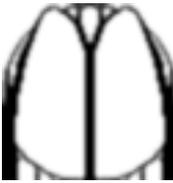 | 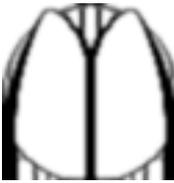 | 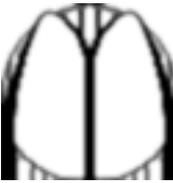 | 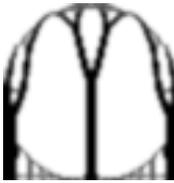 |
| 0.0 / 0.8                                                                          | 0.047 / 0.8                                                                         | 0.155 / 0.9                                                                         | 0.429 / 1.1                                                                         | 0.0 / 0.8                                                                            | 0.001 / 0.8                                                                           | 0.005 / 0.8                                                                           | 0.036 / 0.8                                                                           |
| hoop_64x128_0.2                                                                    |                                                                                     |                                                                                     |                                                                                     |                                                                                      |                                                                                       |                                                                                       |                                                                                       |
| 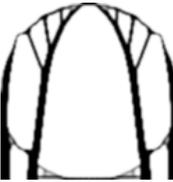 | 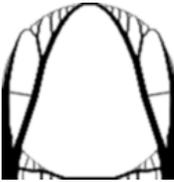 | 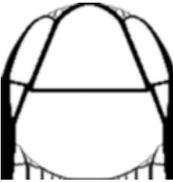 | 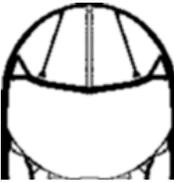 | 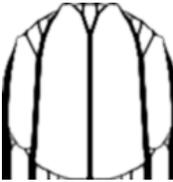 | 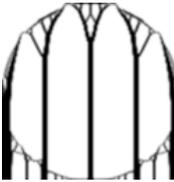 | 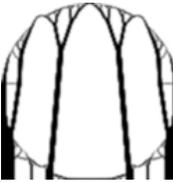 | 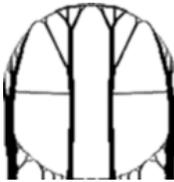 |
| 0.0 / 0.9                                                                          | 0.051 / 0.9                                                                         | 0.169 / 1.1                                                                         | 0.836 / 1.7                                                                         | 0.003 / 0.9                                                                          | 0.0 / 0.9                                                                             | 0.013 / 0.9                                                                           | 0.128 / 1.0                                                                           |
| lshape_0.2_128x128_0.3                                                             |                                                                                     |                                                                                     |                                                                                     |                                                                                      |                                                                                       |                                                                                       |                                                                                       |
| 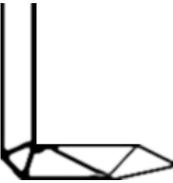 | 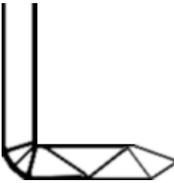 | 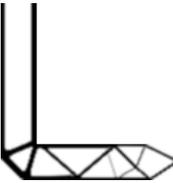 | 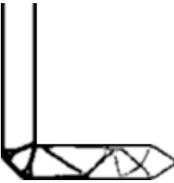 | 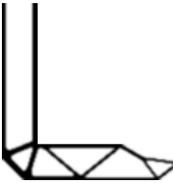 | 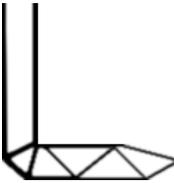 | 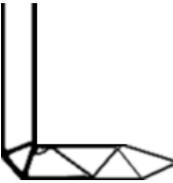 | 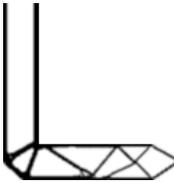 |
| 0.012 / 3062.6                                                                     | 0.0 / 3025.4                                                                        | 0.007 / 3045.3                                                                      | 0.083 / 3277.1                                                                      | 0.002 / 3001.4                                                                       | 0.0 / 2996.0                                                                          | 0.013 / 3036.1                                                                        | 0.029 / 3083.4                                                                        |

| Typical sample          |                |                |                | Best of ensemble |                |                |                |
|-------------------------|----------------|----------------|----------------|------------------|----------------|----------------|----------------|
| CNN-LBFGS               | MMA            | OC             | Pixel-LBFGS    | CNN-LBFGS        | MMA            | OC             | Pixel-LBFGS    |
| l_shape_0.2_256x256_0.2 |                |                |                |                  |                |                |                |
|                         |                |                |                |                  |                |                |                |
| 0.016 / 4390.0          | 0.0 / 4322.7   | 0.009 / 4360.2 | 0.148 / 4960.4 | 0.0 / 4273.5     | 0.008 / 4308.6 | 0.02 / 4360.2  | 0.156 / 4941.8 |
| l_shape_0.2_64x64_0.4   |                |                |                |                  |                |                |                |
|                         |                |                |                |                  |                |                |                |
| 0.015 / 2733.7          | 0.0 / 2693.7   | 0.001 / 2695.3 | 0.048 / 2821.7 | 0.001 / 2690.0   | 0.002 / 2693.2 | 0.0 / 2687.5   | 0.017 / 2733.7 |
| l_shape_0.4_128x128_0.3 |                |                |                |                  |                |                |                |
|                         |                |                |                |                  |                |                |                |
| 0.009 / 292.6           | 0.0 / 290.1    | 0.02 / 295.9   | 0.163 / 337.4  | 0.0 / 286.7      | 0.001 / 287.0  | 0.027 / 294.4  | 0.064 / 305.2  |
| l_shape_0.4_256x256_0.2 |                |                |                |                  |                |                |                |
|                         |                |                |                |                  |                |                |                |
| 0.0 / 409.4             | 0.003 / 410.6  | 0.023 / 418.9  | 0.348 / 551.9  | 0.0 / 399.4      | 0.002 / 400.1  | 0.049 / 418.9  | 0.175 / 469.3  |
| l_shape_0.4_64x64_0.4   |                |                |                |                  |                |                |                |
|                         |                |                |                |                  |                |                |                |
| 0.023 / 227.2           | 0.007 / 223.5  | 0.0 / 222.0    | 0.06 / 235.4   | 0.0 / 220.6      | 0.001 / 220.8  | 0.006 / 221.8  | 0.009 / 222.6  |
| mbb_beam_192x32_0.5     |                |                |                |                  |                |                |                |
|                         |                |                |                |                  |                |                |                |
| 0.0 / 1233.0            | 0.003 / 1236.1 | 0.009 / 1243.6 | 0.095 / 1350.3 | 0.0 / 1220.4     | 0.002 / 1222.7 | 0.009 / 1231.4 | 0.025 / 1250.3 |
| mbb_beam_192x64_0.4     |                |                |                |                  |                |                |                |
|                         |                |                |                |                  |                |                |                |
| 0.0 / 240.9             | 0.008 / 242.9  | 0.017 / 245.1  | 0.16 / 279.4   | 0.0 / 238.0      | 0.0 / 237.9    | 0.014 / 241.2  | 0.039 / 247.3  |
| mbb_beam_384x128_0.3    |                |                |                |                  |                |                |                |
|                         |                |                |                |                  |                |                |                |
| 0.006 / 302.7           | 0.0 / 301.0    | 0.054 / 317.2  | 0.366 / 411.1  | 0.0 / 295.7      | 0.008 / 298.0  | 0.054 / 311.7  | 0.132 / 334.9  |
| mbb_beam_384x64_0.4     |                |                |                |                  |                |                |                |
|                         |                |                |                |                  |                |                |                |
| 0.0 / 1391.0            | 0.001 / 1392.9 | 0.017 / 1415.0 | 0.17 / 1627.0  | 0.0 / 1376.9     | 0.004 / 1382.2 | 0.02 / 1404.7  | 0.067 / 1468.9 |

| Typical sample                                                                     |                                                                                     |                                                                                     |                                                                                     | Best of ensemble                                                                     |                                                                                       |                                                                                       |                                                                                       |
|------------------------------------------------------------------------------------|-------------------------------------------------------------------------------------|-------------------------------------------------------------------------------------|-------------------------------------------------------------------------------------|--------------------------------------------------------------------------------------|---------------------------------------------------------------------------------------|---------------------------------------------------------------------------------------|---------------------------------------------------------------------------------------|
| CNN-LBFGS                                                                          | MMA                                                                                 | OC                                                                                  | Pixel-LBFGS                                                                         | CNN-LBFGS                                                                            | MMA                                                                                   | OC                                                                                    | Pixel-LBFGS                                                                           |
| mbb_beam_96x32_0.5                                                                 |                                                                                     |                                                                                     |                                                                                     |                                                                                      |                                                                                       |                                                                                       |                                                                                       |
| 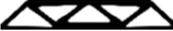   | 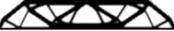   | 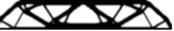   | 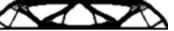   | 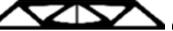   | 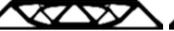   | 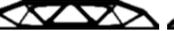   | 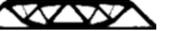   |
| 0.0 / 206.4                                                                        | 0.017 / 209.8                                                                       | 0.02 / 210.5                                                                        | 0.071 / 221.0                                                                       | 0.0 / 205.4                                                                          | 0.002 / 205.8                                                                         | 0.004 / 206.3                                                                         | 0.012 / 208.0                                                                         |
| michell_centered_below_128x128_0.12                                                |                                                                                     |                                                                                     |                                                                                     |                                                                                      |                                                                                       |                                                                                       |                                                                                       |
| 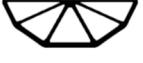  | 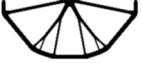   | 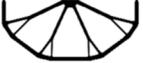   | 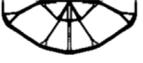   | 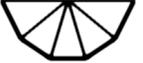    | 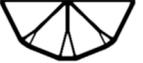   | 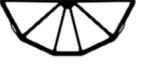   | 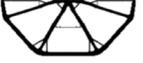   |
| 0.018 / 69.4                                                                       | 0.0 / 68.2                                                                          | 0.015 / 69.2                                                                        | 0.249 / 85.1                                                                        | 0.0 / 65.2                                                                           | 0.01 / 65.9                                                                           | 0.036 / 67.5                                                                          | 0.096 / 71.4                                                                          |
| michell_centered_below_256x256_0.06                                                |                                                                                     |                                                                                     |                                                                                     |                                                                                      |                                                                                       |                                                                                       |                                                                                       |
| 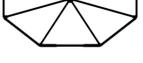  | 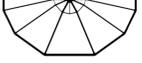   | 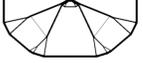   | 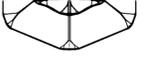   | 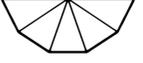    | 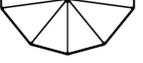   | 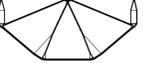   | 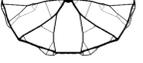   |
| 0.026 / 143.8                                                                      | 0.0 / 140.1                                                                         | 0.084 / 151.9                                                                       | 1.193 / 307.3                                                                       | 0.0 / 131.1                                                                          | 0.028 / 134.7                                                                         | 0.121 / 146.9                                                                         | 0.473 / 193.1                                                                         |
| michell_centered_below_256x256_0.12                                                |                                                                                     |                                                                                     |                                                                                     |                                                                                      |                                                                                       |                                                                                       |                                                                                       |
| 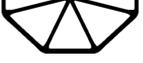  | 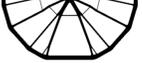   | 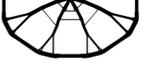   | 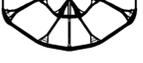   | 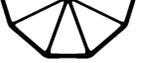    | 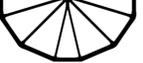   | 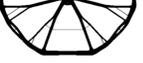   | 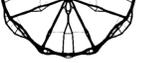   |
| 0.006 / 62.1                                                                       | 0.0 / 61.7                                                                          | 0.043 / 64.3                                                                        | 0.353 / 83.5                                                                        | 0.0 / 59.9                                                                           | 0.0 / 59.8                                                                            | 0.063 / 63.6                                                                          | 0.184 / 70.9                                                                          |
| michell_centered_below_64x64_0.12                                                  |                                                                                     |                                                                                     |                                                                                     |                                                                                      |                                                                                       |                                                                                       |                                                                                       |
| 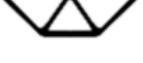  | 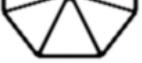   | 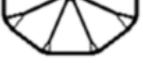   | 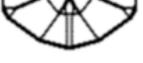   | 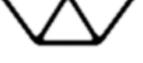    | 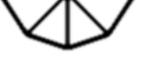   | 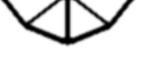   | 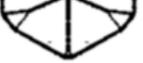   |
| 0.0 / 87.2                                                                         | 0.0 / 87.2                                                                          | 0.044 / 91.0                                                                        | 0.194 / 104.1                                                                       | 0.0 / 80.4                                                                           | 0.007 / 81.0                                                                          | 0.05 / 84.4                                                                           | 0.144 / 92.0                                                                          |
| michell_centered_both_128x256_0.06                                                 |                                                                                     |                                                                                     |                                                                                     |                                                                                      |                                                                                       |                                                                                       |                                                                                       |
| 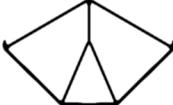 | 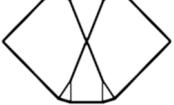 | 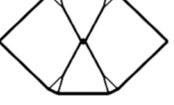 | 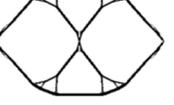 | 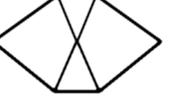 | 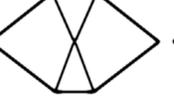 | 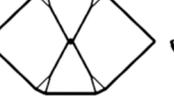 | 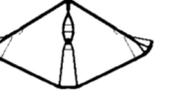 |
| 0.031 / 81.6                                                                       | 0.007 / 79.7                                                                        | 0.0 / 79.1                                                                          | 0.386 / 109.7                                                                       | 0.0 / 74.0                                                                           | 0.002 / 74.1                                                                          | 0.07 / 79.1                                                                           | 0.342 / 99.3                                                                          |
| michell_centered_both_128x256_0.12                                                 |                                                                                     |                                                                                     |                                                                                     |                                                                                      |                                                                                       |                                                                                       |                                                                                       |
| 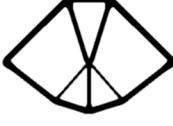 | 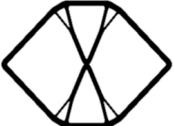 | 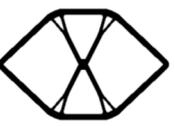 | 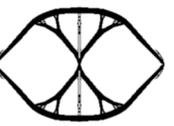 | 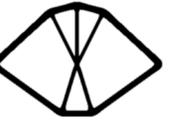 | 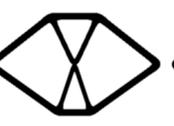 | 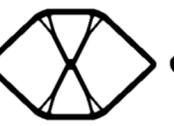 | 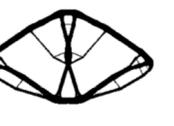 |
| 0.022 / 32.9                                                                       | 0.014 / 32.6                                                                        | 0.0 / 32.2                                                                          | 0.297 / 41.7                                                                        | 0.0 / 31.7                                                                           | 0.003 / 31.8                                                                          | 0.016 / 32.2                                                                          | 0.201 / 38.1                                                                          |
| michell_centered_both_32x64_0.12                                                   |                                                                                     |                                                                                     |                                                                                     |                                                                                      |                                                                                       |                                                                                       |                                                                                       |
| 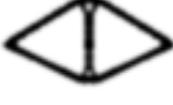 | 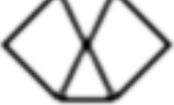 | 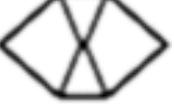 | 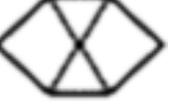 | 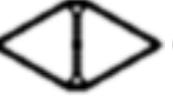 | 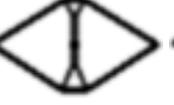 | 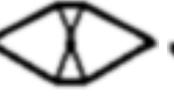 | 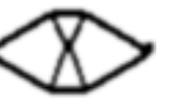 |
| 0.0 / 51.0                                                                         | 0.096 / 55.9                                                                        | 0.064 / 54.3                                                                        | 0.086 / 55.4                                                                        | 0.0 / 50.0                                                                           | 0.0 / 50.0                                                                            | 0.022 / 51.1                                                                          | 0.064 / 53.2                                                                          |

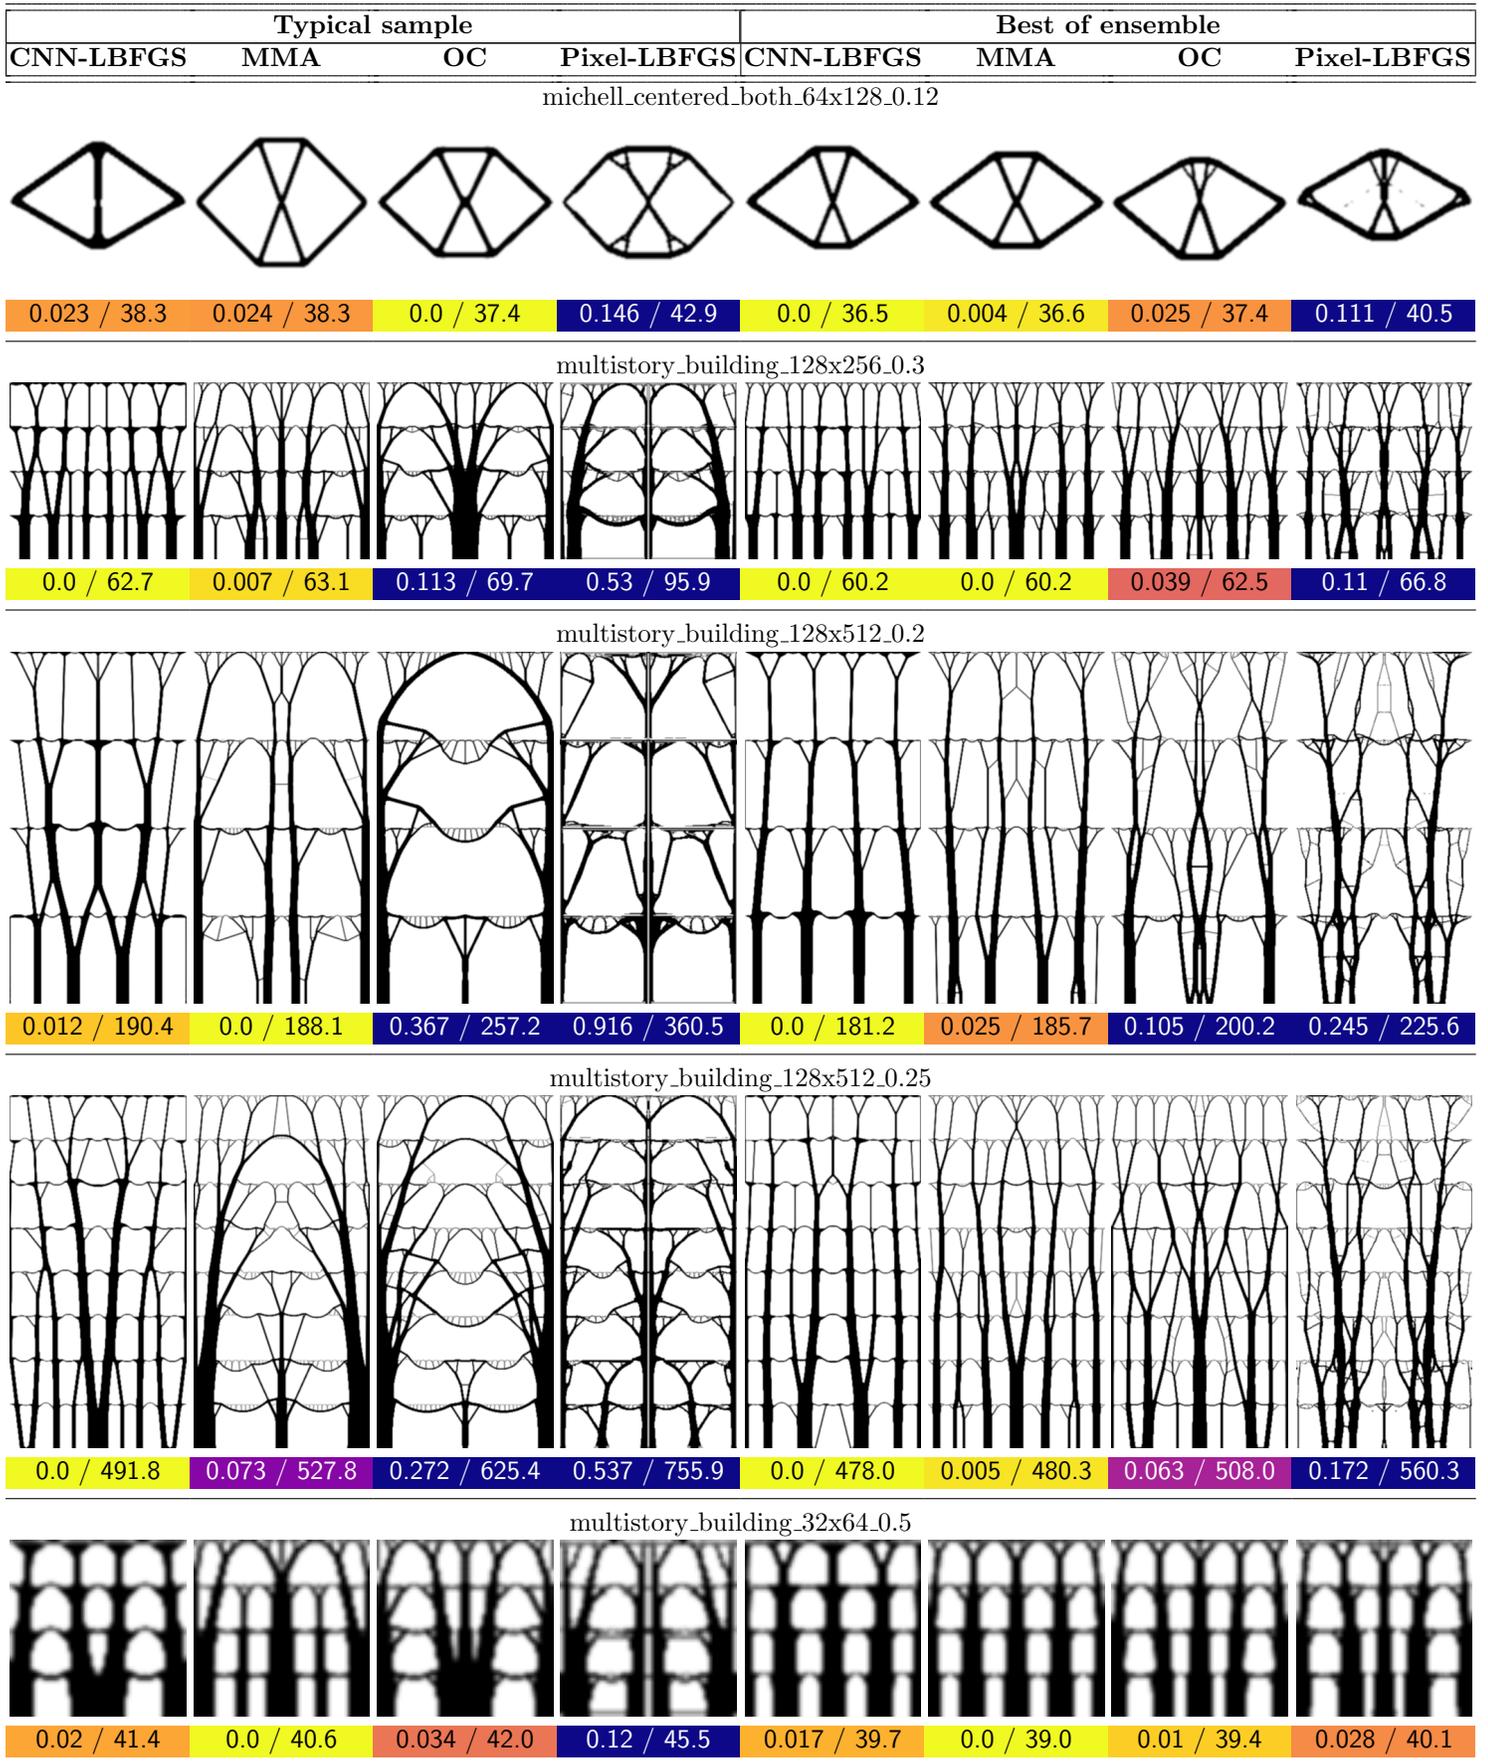

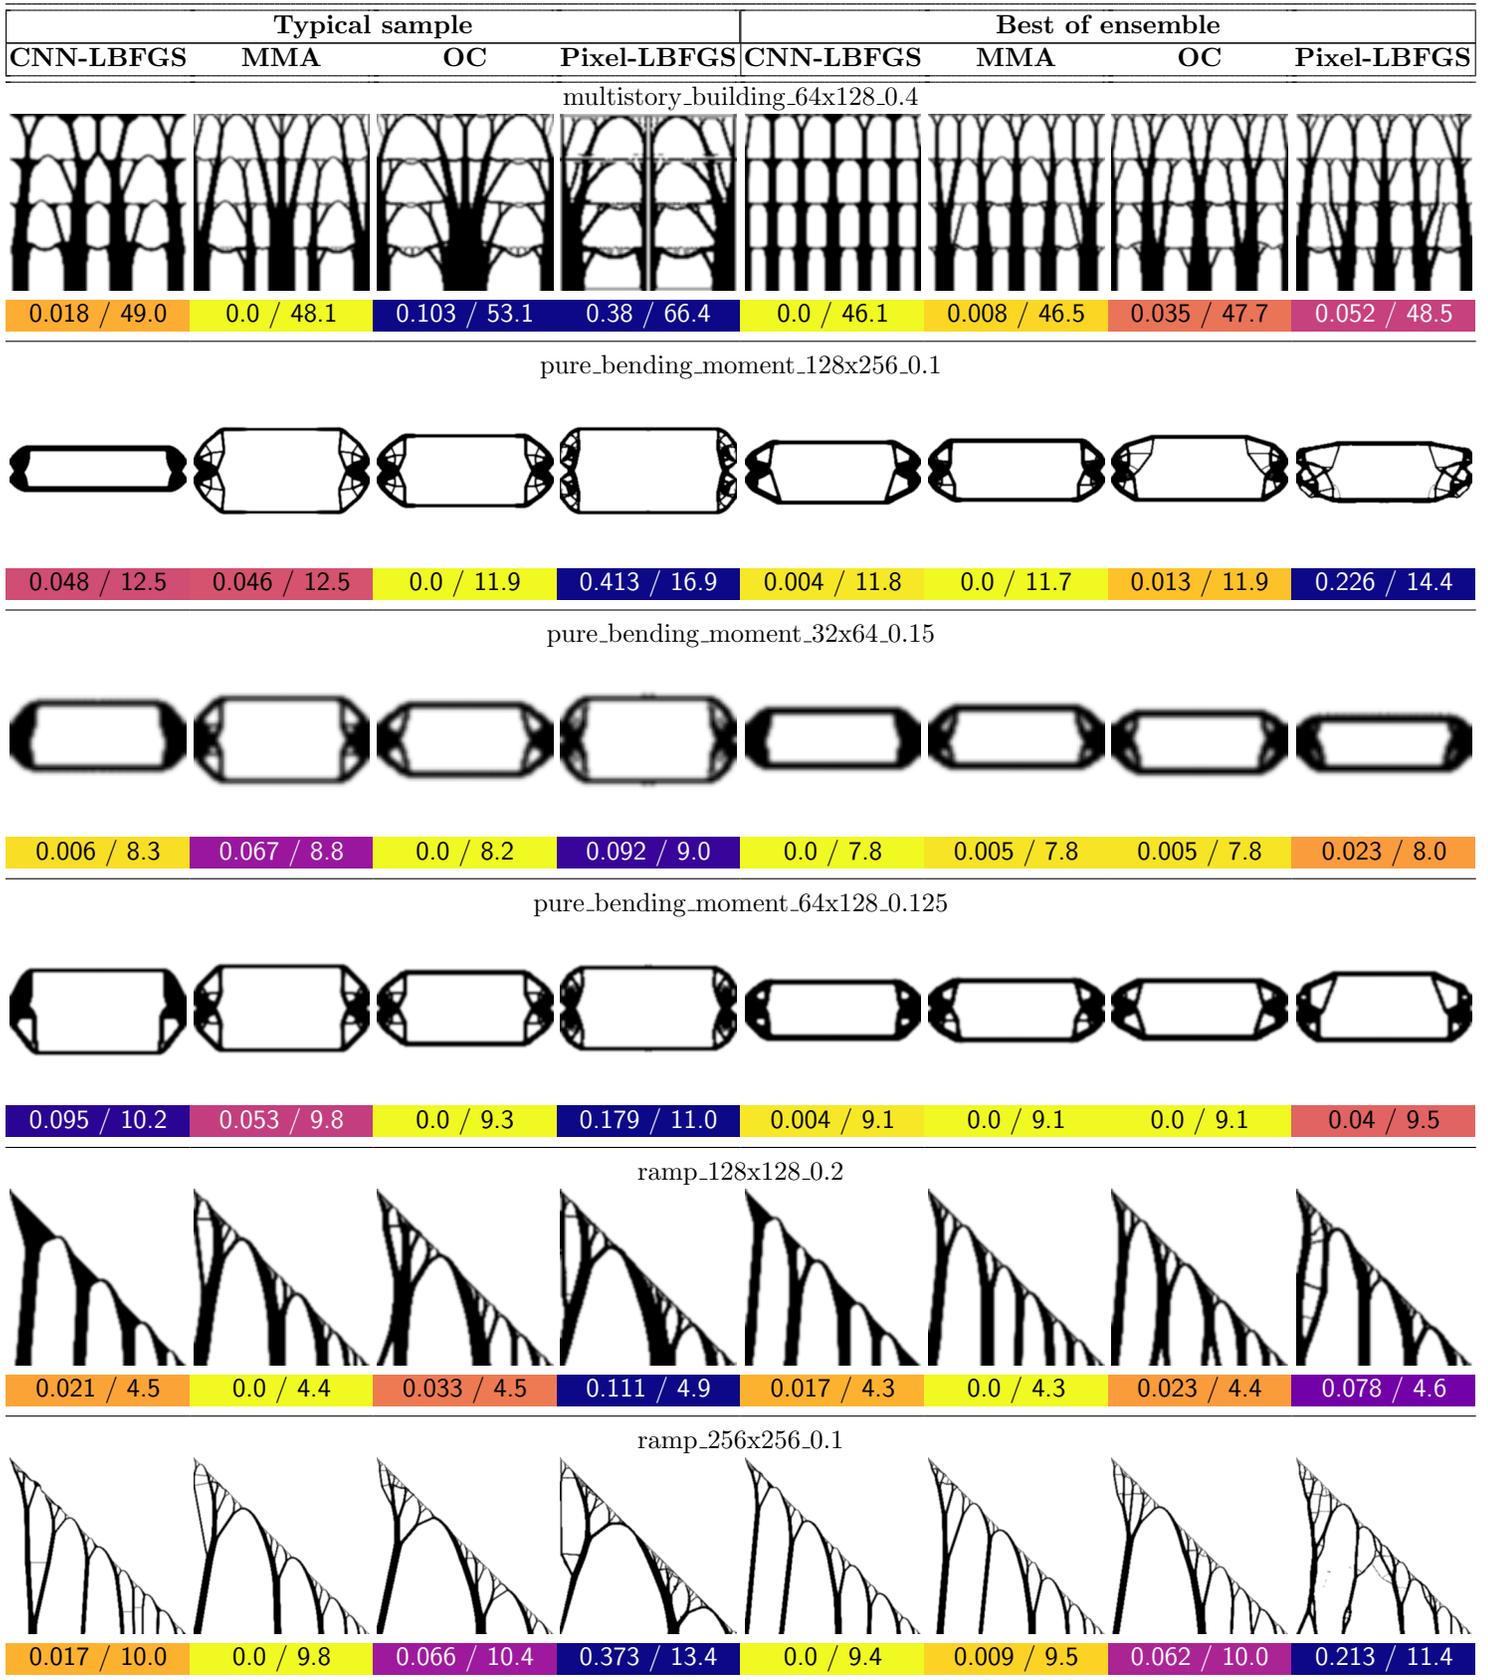

| Typical sample                                                                     |                                                                                     |                                                                                     |                                                                                     | Best of ensemble                                                                     |                                                                                       |                                                                                       |                                                                                       |
|------------------------------------------------------------------------------------|-------------------------------------------------------------------------------------|-------------------------------------------------------------------------------------|-------------------------------------------------------------------------------------|--------------------------------------------------------------------------------------|---------------------------------------------------------------------------------------|---------------------------------------------------------------------------------------|---------------------------------------------------------------------------------------|
| CNN-LBFGS                                                                          | MMA                                                                                 | OC                                                                                  | Pixel-LBFGS                                                                         | CNN-LBFGS                                                                            | MMA                                                                                   | OC                                                                                    | Pixel-LBFGS                                                                           |
| ramp_256x256_0.2                                                                   |                                                                                     |                                                                                     |                                                                                     |                                                                                      |                                                                                       |                                                                                       |                                                                                       |
| 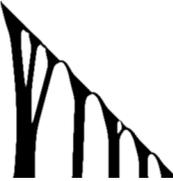   | 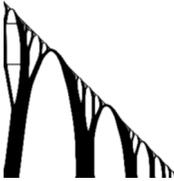   | 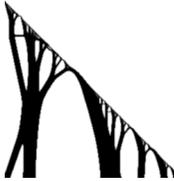   | 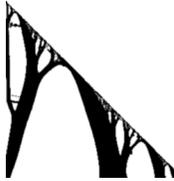   | 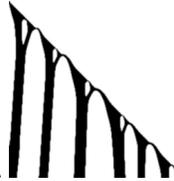   | 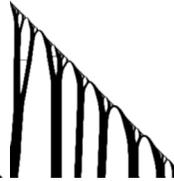   | 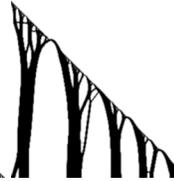   | 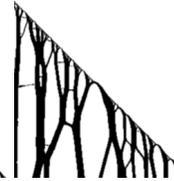   |
| 0.011 / 3.9                                                                        | 0.0 / 3.9                                                                           | 0.053 / 4.1                                                                         | 0.201 / 4.7                                                                         | 0.0 / 3.8                                                                            | 0.001 / 3.8                                                                           | 0.027 / 3.9                                                                           | 0.12 / 4.3                                                                            |
| ramp_64x64_0.3                                                                     |                                                                                     |                                                                                     |                                                                                     |                                                                                      |                                                                                       |                                                                                       |                                                                                       |
| 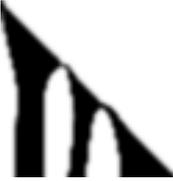   | 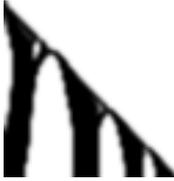   | 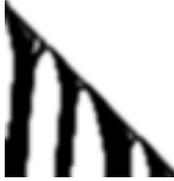   | 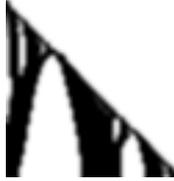   | 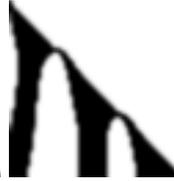   | 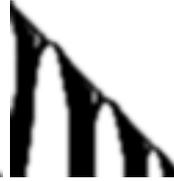   | 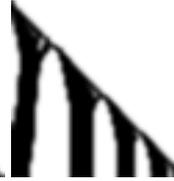   | 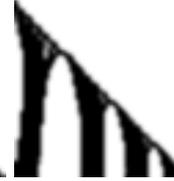   |
| 0.04 / 2.9                                                                         | 0.0 / 2.8                                                                           | 0.014 / 2.8                                                                         | 0.043 / 2.9                                                                         | 0.01 / 2.8                                                                           | 0.0 / 2.8                                                                             | 0.002 / 2.8                                                                           | 0.009 / 2.8                                                                           |
| roof_128x128_0.15                                                                  |                                                                                     |                                                                                     |                                                                                     |                                                                                      |                                                                                       |                                                                                       |                                                                                       |
| 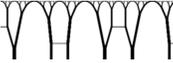   | 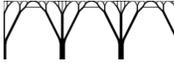   | 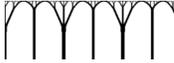   | 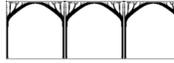   | 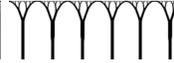   | 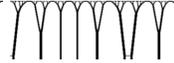   | 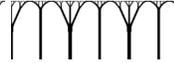   | 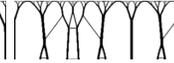   |
| 0.042 / 11.8                                                                       | 0.164 / 13.1                                                                        | 0.0 / 11.3                                                                          | 1.038 / 23.0                                                                        | 0.0 / 11.0                                                                           | 0.04 / 11.5                                                                           | 0.025 / 11.3                                                                          | 0.202 / 13.2                                                                          |
| roof_256x256_0.1                                                                   |                                                                                     |                                                                                     |                                                                                     |                                                                                      |                                                                                       |                                                                                       |                                                                                       |
| 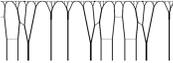   | 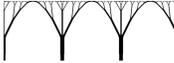   | 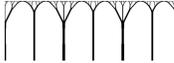   | 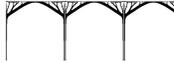   | 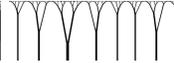   | 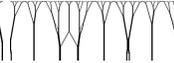   | 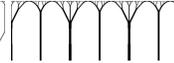   | 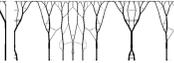   |
| 0.069 / 17.3                                                                       | 0.143 / 18.5                                                                        | 0.0 / 16.2                                                                          | 1.981 / 48.3                                                                        | 0.0 / 15.7                                                                           | 0.072 / 16.9                                                                          | 0.029 / 16.2                                                                          | 0.46 / 23.0                                                                           |
| roof_256x256_0.2                                                                   |                                                                                     |                                                                                     |                                                                                     |                                                                                      |                                                                                       |                                                                                       |                                                                                       |
| 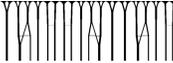 | 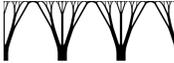 | 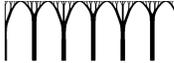 | 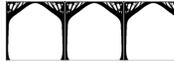 | 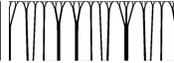 | 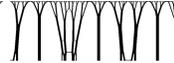 | 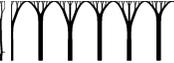 | 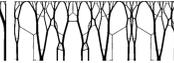 |
| 0.023 / 6.9                                                                        | 0.086 / 7.3                                                                         | 0.0 / 6.7                                                                           | 1.071 / 13.9                                                                        | 0.0 / 6.5                                                                            | 0.029 / 6.7                                                                           | 0.033 / 6.7                                                                           | 0.262 / 8.2                                                                           |
| roof_256x256_0.4                                                                   |                                                                                     |                                                                                     |                                                                                     |                                                                                      |                                                                                       |                                                                                       |                                                                                       |
| 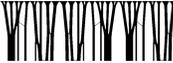 | 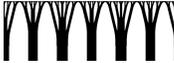 | 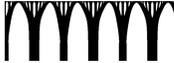 | 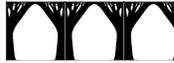 | 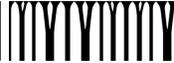 | 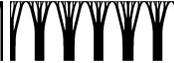 | 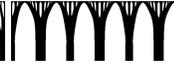 | 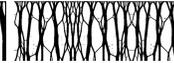 |
| 0.03 / 2.9                                                                         | 0.0 / 2.8                                                                           | 0.035 / 2.9                                                                         | 0.481 / 4.2                                                                         | 0.0 / 2.8                                                                            | 0.004 / 2.8                                                                           | 0.039 / 2.9                                                                           | 0.166 / 3.3                                                                           |
| roof_64x64_0.2                                                                     |                                                                                     |                                                                                     |                                                                                     |                                                                                      |                                                                                       |                                                                                       |                                                                                       |
| 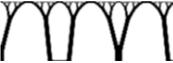 | 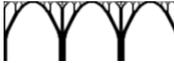 | 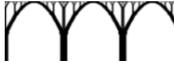 | 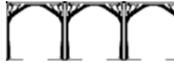 | 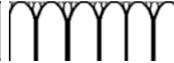 | 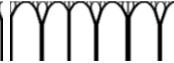 | 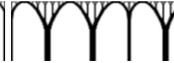 | 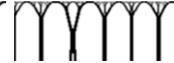 |
| 0.0 / 9.9                                                                          | 0.039 / 10.3                                                                        | 0.054 / 10.4                                                                        | 0.802 / 17.9                                                                        | 0.0 / 9.1                                                                            | 0.007 / 9.2                                                                           | 0.055 / 9.6                                                                           | 0.042 / 9.5                                                                           |
| staggered_points_128x128_0.3                                                       |                                                                                     |                                                                                     |                                                                                     |                                                                                      |                                                                                       |                                                                                       |                                                                                       |
| 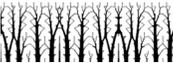 | 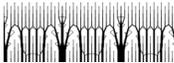 | 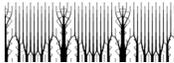 | 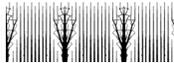 | 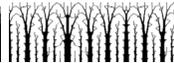 | 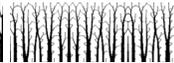 | 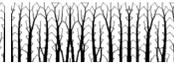 | 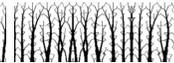 |
| 0.0 / 8.1                                                                          | 0.007 / 8.2                                                                         | 0.043 / 8.5                                                                         | 0.125 / 9.2                                                                         | 0.0 / 7.7                                                                            | 0.004 / 7.8                                                                           | 0.038 / 8.0                                                                           | 0.091 / 8.4                                                                           |
| staggered_points_128x256_0.3                                                       |                                                                                     |                                                                                     |                                                                                     |                                                                                      |                                                                                       |                                                                                       |                                                                                       |
| 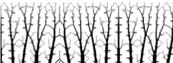 | 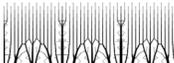 | 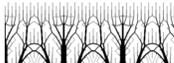 | 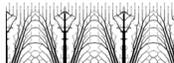 | 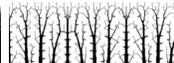 | 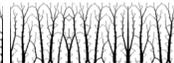 | 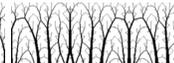 | 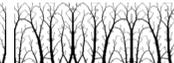 |
| 0.005 / 13.9                                                                       | 0.0 / 13.8                                                                          | 0.086 / 15.0                                                                        | 0.286 / 17.8                                                                        | 0.0 / 13.4                                                                           | 0.007 / 13.5                                                                          | 0.037 / 13.9                                                                          | 0.105 / 14.8                                                                          |

| Typical sample                                                                     |                                                                                     |                                                                                     |                                                                                     | Best of ensemble                                                                    |                                                                                      |                                                                                       |                                                                                       |
|------------------------------------------------------------------------------------|-------------------------------------------------------------------------------------|-------------------------------------------------------------------------------------|-------------------------------------------------------------------------------------|-------------------------------------------------------------------------------------|--------------------------------------------------------------------------------------|---------------------------------------------------------------------------------------|---------------------------------------------------------------------------------------|
| CNN-LBFGS                                                                          | MMA                                                                                 | OC                                                                                  | Pixel-LBFGS                                                                         | CNN-LBFGS                                                                           | MMA                                                                                  | OC                                                                                    | Pixel-LBFGS                                                                           |
| staggered_points_128x512_0.15                                                      |                                                                                     |                                                                                     |                                                                                     |                                                                                     |                                                                                      |                                                                                       |                                                                                       |
| 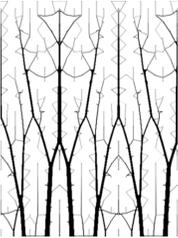   | 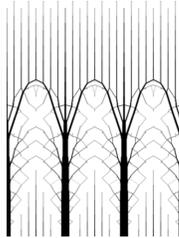   | 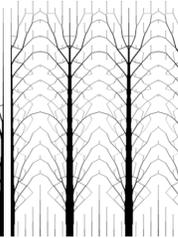   | 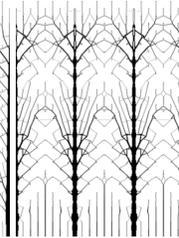   | 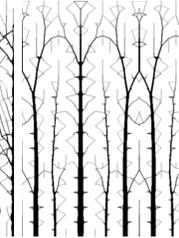   | 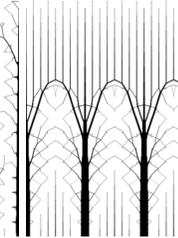   | 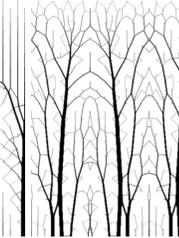   | 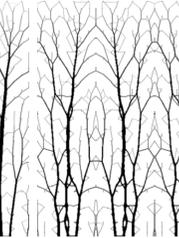   |
| 0.03 / 75.2                                                                        | 0.0 / 73.0                                                                          | 0.094 / 79.8                                                                        | 0.398 / 102.0                                                                       | 0.0 / 71.0                                                                          | 0.027 / 73.0                                                                         | 0.091 / 77.5                                                                          | 0.277 / 90.7                                                                          |
| staggered_points_128x512_0.3                                                       |                                                                                     |                                                                                     |                                                                                     |                                                                                     |                                                                                      |                                                                                       |                                                                                       |
| 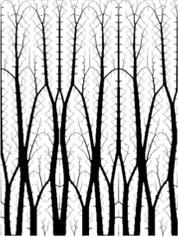   | 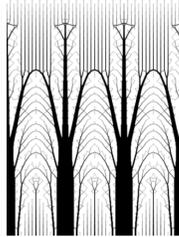   | 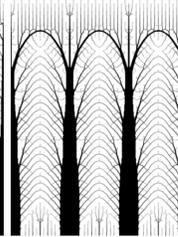   | 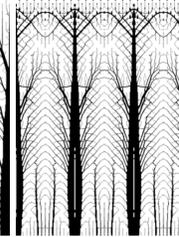   | 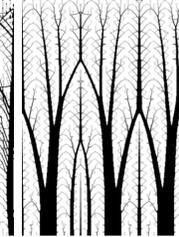   | 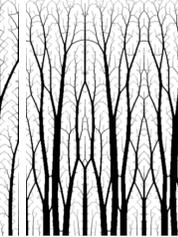   | 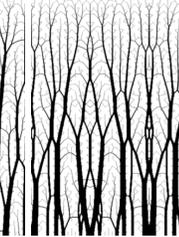   | 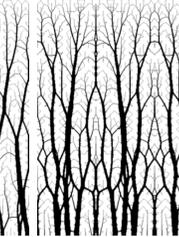   |
| 0.0 / 24.6                                                                         | 0.014 / 24.9                                                                        | 0.047 / 25.8                                                                        | 0.304 / 32.1                                                                        | 0.0 / 23.9                                                                          | 0.022 / 24.5                                                                         | 0.042 / 24.9                                                                          | 0.106 / 26.5                                                                          |
| staggered_points_256x256_0.3                                                       |                                                                                     |                                                                                     |                                                                                     |                                                                                     |                                                                                      |                                                                                       |                                                                                       |
| 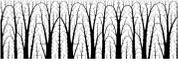   | 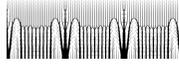   | 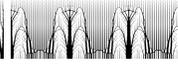   | 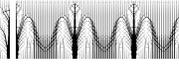   | 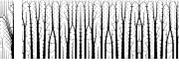   | 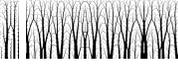   | 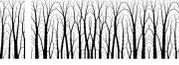   | 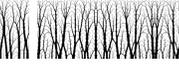   |
| 0.0 / 6.5                                                                          | 0.018 / 6.7                                                                         | 0.129 / 7.4                                                                         | 0.271 / 8.3                                                                         | 0.0 / 6.3                                                                           | 0.017 / 6.4                                                                          | 0.041 / 6.6                                                                           | 0.108 / 7.0                                                                           |
| staggered_points_256x256_0.5                                                       |                                                                                     |                                                                                     |                                                                                     |                                                                                     |                                                                                      |                                                                                       |                                                                                       |
| 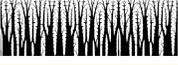 | 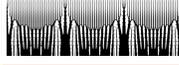 | 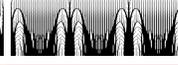 | 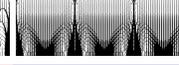 | 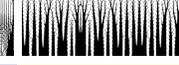 | 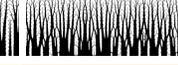 | 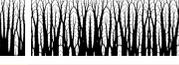 | 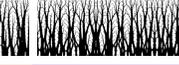 |
| 0.0 / 2.9                                                                          | 0.032 / 3.0                                                                         | 0.042 / 3.0                                                                         | 0.163 / 3.4                                                                         | 0.0 / 2.9                                                                           | 0.015 / 2.9                                                                          | 0.035 / 3.0                                                                           | 0.079 / 3.1                                                                           |
| staggered_points_32x128_0.3                                                        |                                                                                     |                                                                                     |                                                                                     |                                                                                     |                                                                                      |                                                                                       |                                                                                       |
| 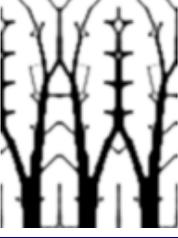 | 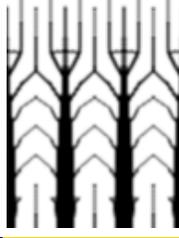 | 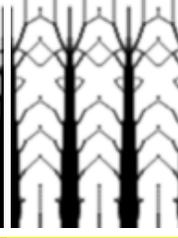 | 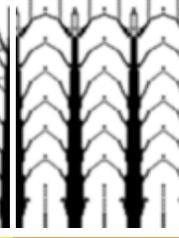 | 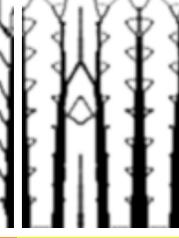 | 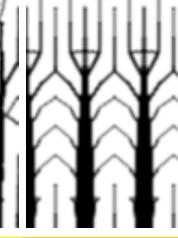 | 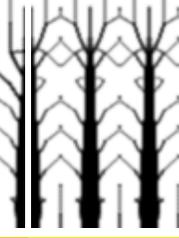 | 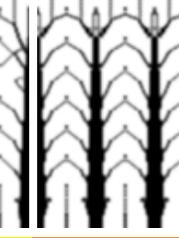 |
| 0.103 / 45.6                                                                       | 0.008 / 41.7                                                                        | 0.0 / 41.3                                                                          | 0.023 / 42.3                                                                        | 0.0 / 41.2                                                                          | 0.012 / 41.7                                                                         | 0.003 / 41.3                                                                          | 0.026 / 42.3                                                                          |
| staggered_points_64x128_0.3                                                        |                                                                                     |                                                                                     |                                                                                     |                                                                                     |                                                                                      |                                                                                       |                                                                                       |
| 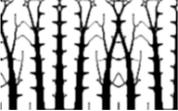 | 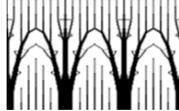 | 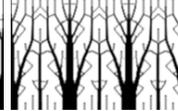 | 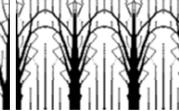 | 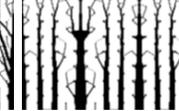 | 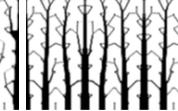 | 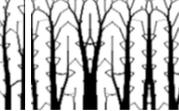 | 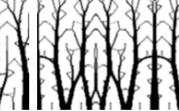 |
| 0.034 / 18.2                                                                       | 0.0 / 17.6                                                                          | 0.073 / 18.9                                                                        | 0.189 / 21.0                                                                        | 0.0 / 16.7                                                                          | 0.011 / 16.9                                                                         | 0.064 / 17.8                                                                          | 0.115 / 18.6                                                                          |
| staggered_points_64x256_0.3                                                        |                                                                                     |                                                                                     |                                                                                     |                                                                                     |                                                                                      |                                                                                       |                                                                                       |
| 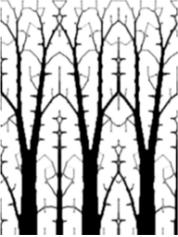 | 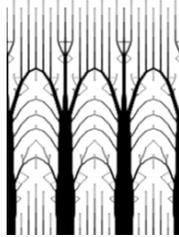 | 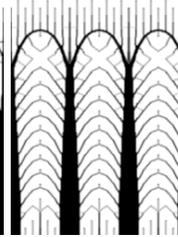 | 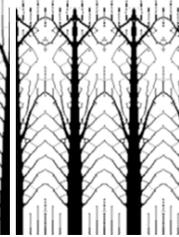 | 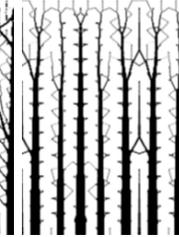 | 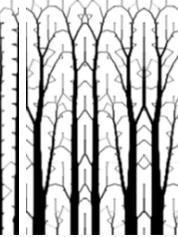 | 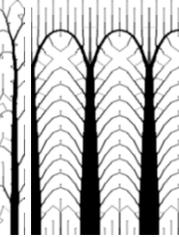 | 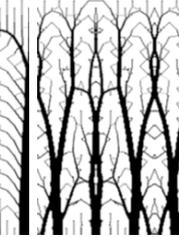 |
| 0.025 / 31.3                                                                       | 0.001 / 30.5                                                                        | 0.0 / 30.5                                                                          | 0.181 / 36.0                                                                        | 0.0 / 29.2                                                                          | 0.031 / 30.2                                                                         | 0.043 / 30.5                                                                          | 0.117 / 32.7                                                                          |

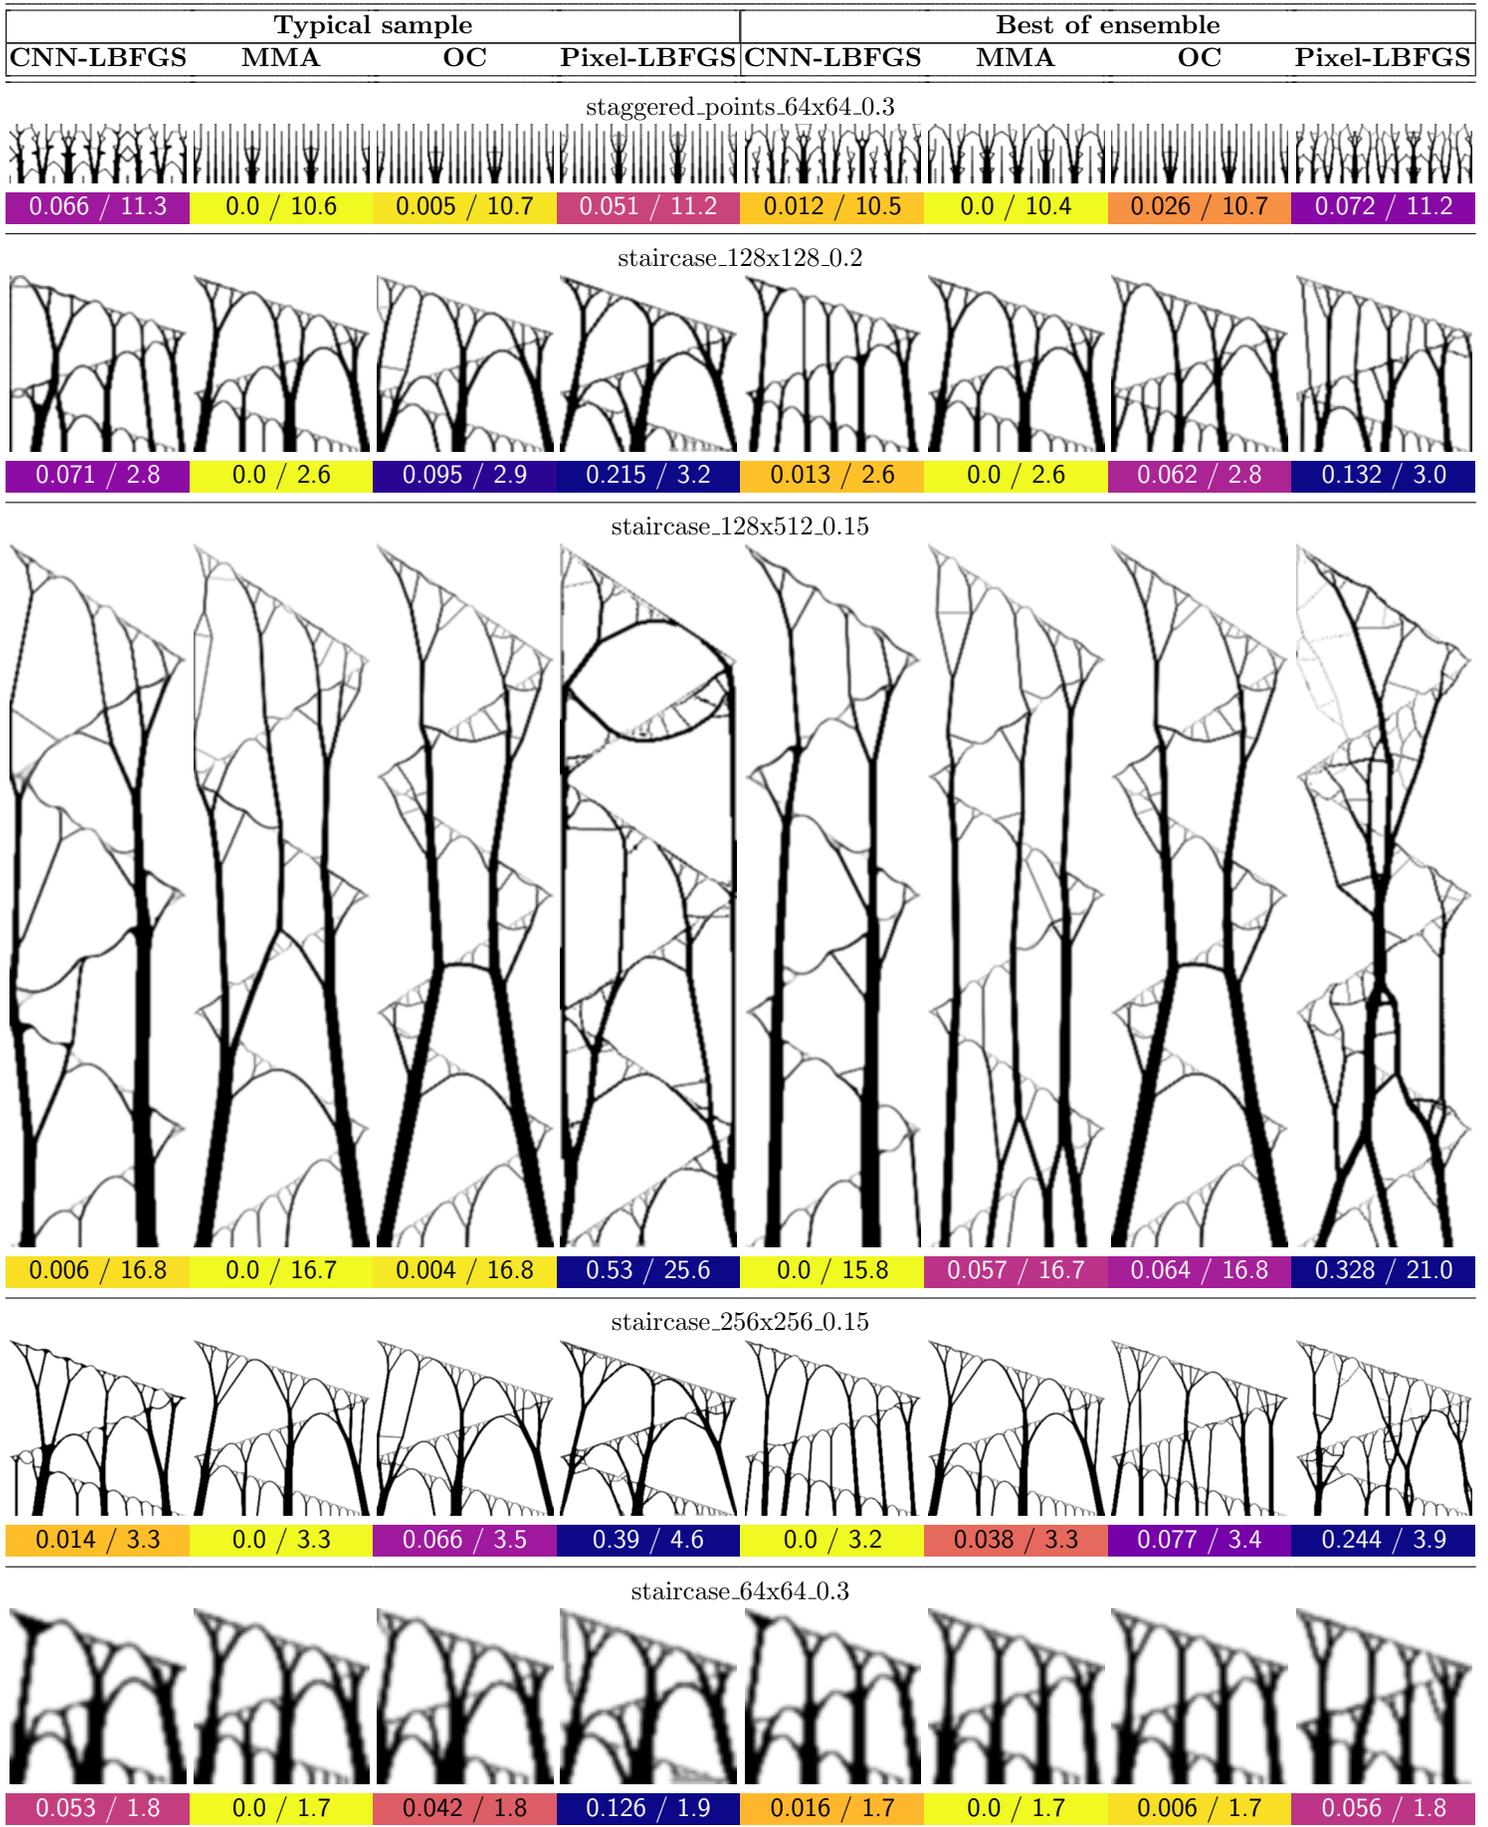

| Typical sample                   |              |               |               | Best of ensemble |               |               |               |
|----------------------------------|--------------|---------------|---------------|------------------|---------------|---------------|---------------|
| CNN-LBFGS                        | MMA          | OC            | Pixel-LBFGS   | CNN-LBFGS        | MMA           | OC            | Pixel-LBFGS   |
| thin_support_bridge_128x128_0.2  |              |               |               |                  |               |               |               |
|                                  |              |               |               |                  |               |               |               |
| 0.0 / 78.1                       | 0.033 / 80.8 | 0.072 / 83.8  | 0.341 / 104.8 | 0.0 / 75.8       | 0.006 / 76.2  | 0.016 / 77.0  | 0.04 / 78.8   |
| thin_support_bridge_256x256_0.1  |              |               |               |                  |               |               |               |
|                                  |              |               |               |                  |               |               |               |
| 0.025 / 170.4                    | 0.0 / 166.2  | 0.115 / 185.3 | 0.597 / 265.3 | 0.0 / 156.7      | 0.061 / 166.1 | 0.127 / 176.5 | 0.301 / 203.8 |
| thin_support_bridge_256x256_0.15 |              |               |               |                  |               |               |               |
|                                  |              |               |               |                  |               |               |               |
| 0.002 / 96.7                     | 0.0 / 96.5   | 0.018 / 98.2  | 0.379 / 133.1 | 0.0 / 92.2       | 0.018 / 93.9  | 0.065 / 98.2  | 0.194 / 110.1 |
| thin_support_bridge_64x64_0.3    |              |               |               |                  |               |               |               |
|                                  |              |               |               |                  |               |               |               |
| 0.0 / 54.9                       | 0.057 / 58.0 | 0.141 / 62.7  | 0.121 / 61.6  | 0.0 / 53.6       | 0.001 / 53.6  | 0.001 / 53.6  | 0.019 / 54.6  |
| two_level_bridge_128x128_0.16    |              |               |               |                  |               |               |               |
|                                  |              |               |               |                  |               |               |               |
| 0.018 / 22.7                     | 0.0 / 22.4   | 0.0 / 22.3    | 0.127 / 25.2  | 0.002 / 21.9     | 0.0 / 21.9    | 0.013 / 22.2  | 0.064 / 23.3  |
| two_level_bridge_256x256_0.12    |              |               |               |                  |               |               |               |
|                                  |              |               |               |                  |               |               |               |
| 0.004 / 28.8                     | 0.004 / 28.8 | 0.0 / 28.7    | 0.263 / 36.3  | 0.0 / 27.8       | 0.017 / 28.2  | 0.029 / 28.6  | 0.179 / 32.8  |
| two_level_bridge_64x64_0.2       |              |               |               |                  |               |               |               |
|                                  |              |               |               |                  |               |               |               |
| 0.015 / 19.1                     | 0.008 / 18.9 | 0.0 / 18.8    | 0.052 / 19.8  | 0.002 / 18.5     | 0.0 / 18.5    | 0.003 / 18.5  | 0.031 / 19.1  |
